# Supplementary material for: Bound and continuum state $\beta^-$ decay of bare atoms: enhancement of decay rate and changes in $\beta^{-}$ decay branching
Source: arXiv:1808.09717 source file (2019-11-29)
Supplement: Supplementary file 1 [file supplement_10.pdf]

# Bound and continuum state $\beta^-$ decay of bare atoms: enhancement of decay rate and changes in $\beta^-$ decay branching : Supplemental Material

Arkabrata Gupta, Chirashree Lahiri, and S. Sarkar*

*Department of Physics, Indian Institute of Engineering Science and Technology (Formerly, Bengal Engineering and Science University), Shibpur, Howrah-711103, India*

In this supplemental material, we have tabulated rates of $\beta^-$ decay to both continuum and bound states separately for some fully ionized (bare) atoms in the mass range A $\approx$ 60-240. Three tables elaborating the results of $\beta^-$ decay rates for decay to continuum and bound states for 114 transition cases in 27 different nuclei (33 parent levels) have been tabulated and compared with the previously calculated values, if available.

---

**Parameters used** :

• $Q_n$ : Neutral atom Q value in keV.
• $R_1$ : the phenomenological radius evaluated as $R_1 = 1.2A^{1/3}$ fm.
• $R_2$ : the nuclear charge radius [I. Angeli and K.P. Marinova, At. Data Nucl. Data Tables **99**, 69 (2013)]
• $R_3$ : the half-density radius $R_3 = (1.123A^{1/3} - 0.941A^{-1/3})$ fm. [N. B. Gove and M. J. Martin, Nucl. Data Tables **10**, 205 (1971)].
• $T_{1/2}$ in the 'Decay Transition' panel -Table 1: the total half-life of the concerned energy level of the parent atom (including all possible decay channels, viz. $\beta$, $\alpha$, IT etc). However, we have tabulated *Log ft* values only for allowed (a), first-forbidden non-unique (nu) and first-forbidden unique (u) transitions.
• $\lambda_B$ and $\lambda_C$ : $\beta^-$ decay rates for bound and continuum states, respectively.
• $\lambda_{Bare}$ and $\lambda_{Neutral}$ : $\beta^-$ decay rates for bare and neutral atoms, respectively. Here, $\lambda_{Bare} = \lambda_B + \lambda_C$.

**References :**

• 'Takahashi' : K. Takahashi, R. N. Boyd, G. J. Mathews, and K. Yokoi, Phys. Rev. C **36**, 1522 (1987).
• 'NNDC': National Nuclear Data Center, (https://www.nndc.bnl.gov/).

---

*Electronic address: Corresponding author: ss@physics.iiests.ac.in

Table 1: Log $f_0t(f_1t)$ values for different choices of radii compared with the results of previous theoretical works and experimental data. Here (-) : no available data for $R_2$ and/or Takahashi, (dashed lines in 'Decay Transition' panel) : higher order forbidden transitions (not calculated here).

| Transition Details | | | | Present Calculation | | | Previous values | |
|---|---|---|---|---|---|---|---|---|
| Decay Transition | Daughter level | Decay Type | $Q_n$ (keV) | $R_1$ (fm)<br>$R_2$ (fm)<br>$R_3$ (fm) | Log $f_0$ (Log $f_1$)$_{R_1}$<br>Log $f_0$ (Log $f_1$)$_{R_2}$<br>Log $f_0$ (Log $f_1$)$_{R_3}$ | Log $f_0t$(Log $f_1t$)$_{R_1}$<br>Log $f_0t$(Log $f_1t$)$_{R_2}$<br>Log $f_0t$(Log $f_1t$)$_{R_3}$ | Takahashi | NNDC |
| 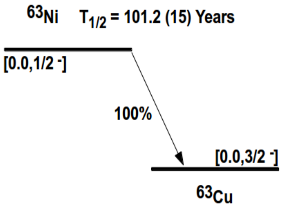 | $\left[0.0, \frac{3}{2}^-\right]$ | (a) | 66.945 | 4.775<br>3.882<br>4.232 | -2.8377<br>-2.8320<br>-2.8360 | 6.665<br>6.671<br>6.667 | 6.64 | 6.7 |
| 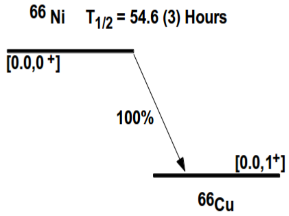 | $[0.0, 1^+]$ | (a) | 251.900 | 4.849<br>-<br>4.305 | -1.0155<br>-<br>-1.0174 | 4.278<br>-<br>4.276 | 4.12 | 4.3 |
| 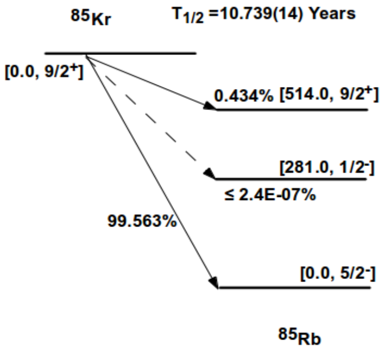 | $\left[0.0, \frac{5}{2}^-\right]$ | (u) | 687.000 | 5.276<br>4.204<br>4.724 | 0.9251<br>0.9307<br>0.9287 | 9.457<br>9.463<br>9.461 | - | 9.446 |
| | $\left[514.0, \frac{9}{2}^+\right]$ | (a) | 173.000 | 5.276<br>4.204<br>4.724 | -1.3777<br>-1.3699<br>-1.3727 | 9.515<br>9.522<br>9.520 | - | 9.51 |
| 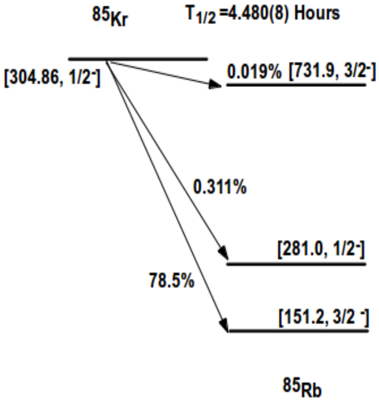 | $\left[151.2, \frac{3}{2}^-\right]$ | (a) | 840.660 | 5.276<br>4.204<br>4.724 | 0.9435<br>0.9513<br>0.9485 | 5.256<br>5.264<br>5.261 | - | 5.250 |
| | $\left[281.0, \frac{1}{2}^-\right]$ | (a) | 710.860 | 5.276<br>4.204<br>4.724 | 0.6785<br>0.6863<br>0.6835 | 7.393<br>7.401<br>7.398 | - | 7.39 |
| | $\left[731.9, \frac{3}{2}^-\right]$ | (a) | 259.960 | 5.276<br>4.204<br>4.724 | -0.8107<br>-0.8029<br>-0.8058 | 7.118<br>7.126<br>7.123 | - | 7.1 |
| 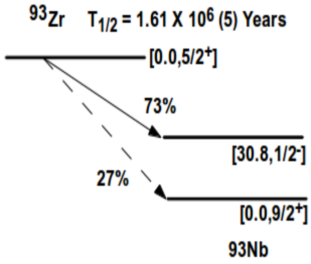 | $\left[30.8, \frac{1}{2}^-\right]$ | (u) | 60.000 | 5.437<br>4.324<br>4.880 | -3.6084<br>-3.6034<br>-3.6068 | 10.234<br>10.239<br>10.235 | (10.0) | 10.17 |

Table 1: (Cotnd.)

| Transition Details | | | | Present Calculation | | | Previous values | |
|---|---|---|---|---|---|---|---|---|
| Decay Transition | Daughter level | Decay Type | $Q_n$ (keV) | $R_1$ (fm)<br>$R_2$ (fm)<br>$R_3$ (fm) | Log $f_0$ (Log $f_1$)$_{R_1}$<br>Log $f_0$ (Log $f_1$)$_{R_2}$<br>Log $f_0$ (Log $f_1$)$_{R_3}$ | Log $f_0t$(Log $f_1t$)$_{R_1}$<br>Log $f_0t$(Log $f_1t$)$_{R_2}$<br>Log $f_0t$(Log $f_1t$)$_{R_3}$ | Takahashi | NNDC |
| 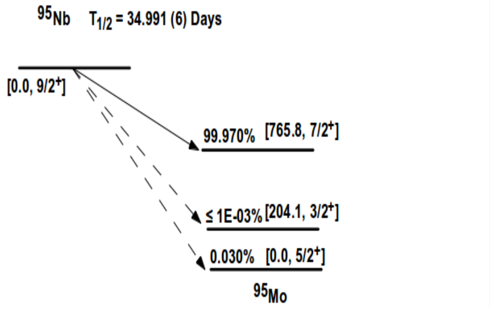 | $\left[765.8, \frac{7}{2}^+\right]$ | (a) | 159.800 | 5.475<br>4.363<br>4.918 | -1.3797<br>-1.3697<br>-1.3766 | 5.101<br>5.111<br>5.104 | 5.09 | 5.091 |
| 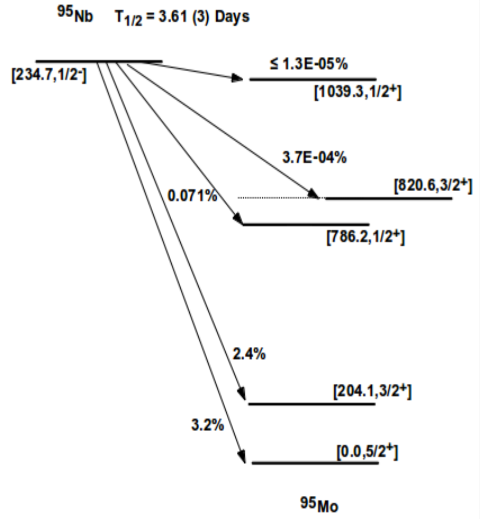 | $\left[0.0, \frac{5}{2}^+\right]$ | (u) | 1160.300 | 5.475<br>4.363<br>4.918 | 2.2274<br>2.2350<br>2.2297 | 9.216<br>9.224<br>9.219 | - | 9.20 |
| | $\left[204.1, \frac{3}{2}^+\right]$ | (nu) | 956.200 | 5.475<br>4.363<br>4.918 | 1.2432<br>1.2533<br>1.2463 | 8.357<br>8.367<br>8.360 | - | 8.4 |
| | $\left[786.2, \frac{1}{2}^+\right]$ | (nu) | 374.100 | 5.475<br>4.363<br>4.918 | -0.1873<br>-0.1772<br>-0.1842 | 8.455<br>8.466<br>8.459 | - | 8.4 |
| | $\left[820.6, \frac{3}{2}^+\right]$ | (nu) | 339.700 | 5.475<br>4.363<br>4.918 | -0.3258<br>-0.3157<br>-0.3227 | 10.600<br>10.610<br>10.603 | - | 10.6 |
| | $\left[1039.3, \frac{1}{2}^+\right]$ | (nu) | 121.000 | 5.475<br>4.363<br>4.918 | -1.7577<br>-1.7476<br>-1.7546 | 10.622<br>10.632<br>10.625 | - | ≥10.3 |
| 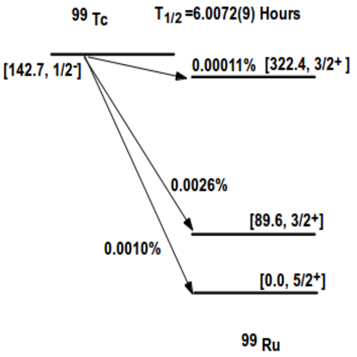 | $\left[0.0, \frac{5}{2}^+\right]$ | (u) | 440.184 | 5.551<br>4.434<br>4.992 | 0.0884<br>0.0960<br>0.0907 | 9.423<br>9.431<br>9.426 | - | 9.38 |
| | $\left[89.6, \frac{3}{2}^+\right]$ | (nu) | 350.584 | 5.551<br>4.434<br>4.992 | -0.2394<br>-0.2283<br>-0.2360 | 8.681<br>8.692<br>8.684 | - | 8.65 |
| | $\left[322.4, \frac{3}{2}^+\right]$ | (nu) | 117.784 | 5.551<br>4.434<br>4.992 | -1.7545<br>-1.7434<br>-1.7511 | 8.540<br>8.550<br>8.543 | - | 8.5 |

Table 1: (Cotnd.)

| Transition Details | | | | Present Calculation | | | Previous values | |
|---|---|---|---|---|---|---|---|---|
| Decay Transition | Daughter level | Decay Type | $Q_n$ (keV) | $R_1$ (fm)<br>$R_2$ (fm)<br>$R_3$ (fm) | Log $f_0$ (Log $f_1)_{R_1}$<br>Log $f_0$ (Log $f_1)_{R_2}$<br>Log $f_0$ (Log $f_1)_{R_3}$ | Log $f_0t$(Log $f_1t)_{R_1}$<br>Log $f_0t$(Log $f_1t)_{R_2}$<br>Log $f_0t$(Log $f_1t)_{R_3}$ | Takahashi | NNDC |
| 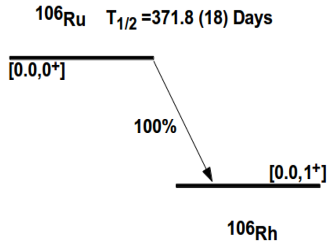 | $[0.0, 1^+]$ | (a) | 39.400 | 5.679<br>-<br>5.116 | -3.1912<br>-<br>-3.1843 | 4.316<br>-<br>4.322 | 4.30 | 4.31 |
| 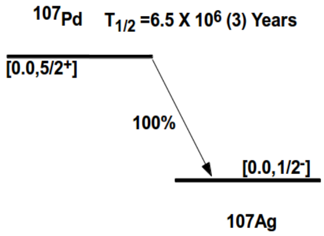 | $\left[0.0, \frac{1}{2}^-\right]$ | (u) | 34.100 | 5.697<br>4.545<br>5.133 | -4.2615<br>-4.2557<br>-4.2578 | 10.050<br>10.056<br>10.054 | 9.93 | 9.9 |
| 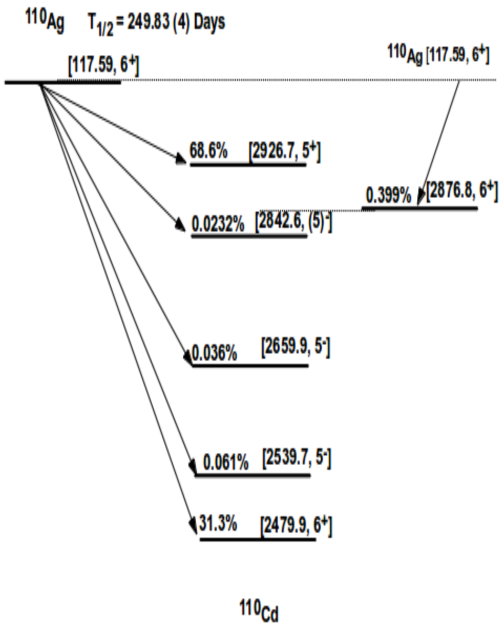 | $[2479.9, 6^+]$ | (a) | 530.590 | 5.750<br>4.577<br>5.184 | 0.4463<br>0.4586<br>0.4541 | 8.285<br>8.297<br>8.293 | - | 8.277 |
| | $[2539.7, 5^-]$ | (nu) | 470.790 | 5.750<br>4.577<br>5.184 | 0.2691<br>0.2814<br>0.2770 | 10.816<br>10.830<br>10.826 | - | 10.81 |
| | $[2659.9, 5^-]$ | (nu) | 350.590 | 5.750<br>4.577<br>5.184 | -0.1586<br>-0.1464<br>-0.1508 | 10.619<br>10.632<br>10.627 | - | 10.61 |
| | $[2842.6, (5)^-]$ | (nu) | 167.890 | 5.750<br>4.577<br>5.184 | -1.1847<br>-1.1724<br>-1.1768 | 9.784<br>9.796<br>9.792 | - | 9.773 |
| | $[2876.8, 6^+]$ | (a) | 133.690 | 5.750<br>4.577<br>5.184 | -1.4943<br>-1.4820<br>-1.4865 | 8.239<br>8.251<br>8.247 | - | 8.228 |
| | $[2926.7, 5^+]$ | (a) | 83.790 | 5.750<br>4.577<br>5.184 | -2.1235<br>-2.1112<br>-2.1156 | 5.374<br>5.387<br>5.382 | 5.37 | 5.365 |

Table 1: (Cotnd.)

| Transition Details | | | | Present Calculation | | | Previous values | |
|---|---|---|---|---|---|---|---|---|
| Decay Transition | Daughter level | Decay Type | $Q_n$ (keV) | $R_1$ (fm)<br>$R_2$ (fm)<br>$R_3$ (fm) | Log $f_0$ (Log $f_1)_{R_1}$<br>Log $f_0$ (Log $f_1)_{R_2}$<br>Log $f_0$ (Log $f_1)_{R_3}$ | Log $f_0t$(Log $f_1t)_{R_1}$<br>Log $f_0t$(Log $f_1t)_{R_2}$<br>Log $f_0t$(Log $f_1t)_{R_3}$ | Takahashi | NNDC |
| 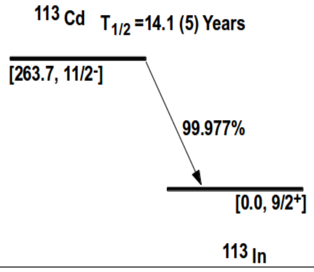 | $\left[0.0, \frac{9}{2}^{+}\right]$ | (nu) | 585.700 | 5.802<br>4.601<br>5.235 | 0.6151<br>0.6280<br>0.6191 | 9.263<br>9.276<br>9.267 | - | 9.25 |
| 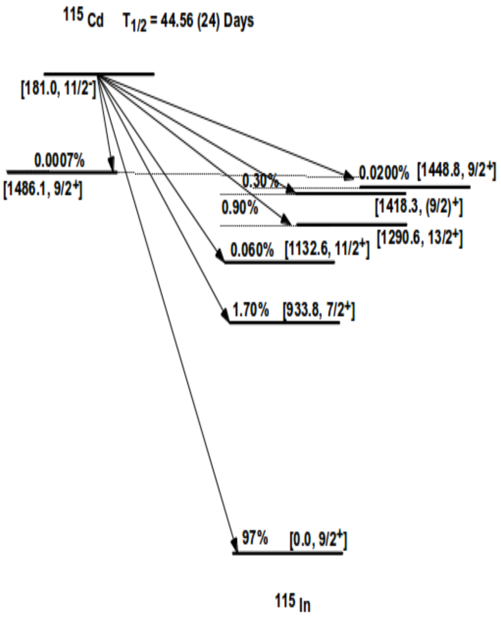 | $\left[0.0, \frac{9}{2}^{+}\right]$ | (nu) | 1629.700 | 5.836<br>4.616<br>5.268 | 2.2569<br>2.2698<br>2.2609 | 8.856<br>8.868<br>8.860 | - | 8.8 |
| | $\left[933.8, \frac{7}{2}^{+}\right]$ | (u) | 695.900 | 5.836<br>4.616<br>5.268 | 1.1738<br>1.1832<br>1.1767 | 9.529<br>9.538<br>9.532 | - | ~9.5 |
| | $\left[1132.6, \frac{11}{2}^{+}\right]$ | (nu) | 497.100 | 5.836<br>4.616<br>5.268 | 0.3710<br>0.3838<br>0.3750 | 10.178<br>10.191<br>10.182 | - | ~10.2 |
| | $\left[1290.6, \frac{13}{2}^{+}\right]$ | (nu) | 339.100 | 5.836<br>4.616<br>5.268 | -0.1840<br>-0.1712<br>-0.1800 | 8.447<br>8.460<br>8.451 | - | ~ 8.4 |
| | $\left[1418.3, \left(\frac{9}{2}\right)^{+}\right]$ | (nu) | 211.400 | 5.836<br>4.616<br>5.268 | -0.8471<br>-0.8343<br>-0.8431 | 8.261<br>8.274<br>8.265 | - | ~ 8.2 |
| | $\left[1448.8, \frac{9}{2}^{+}\right]$ | (nu) | 180.900 | 5.836<br>4.616<br>5.268 | -1.0626<br>-1.0498<br>-1.0586 | 9.222<br>9.235<br>9.226 | - | ~ 9.2 |
| | $\left[1486.1, \frac{9}{2}^{+}\right]$ | (nu) | 143.600 | 5.836<br>4.616<br>5.268 | -1.3775<br>-1.3647<br>-1.3735 | 10.363<br>10.376<br>10.367 | - | ~ 10.3 |

Table 1: (Cotnd.)

| Transition Details | | | | Present Calculation | | | Previous values | |
|---|---|---|---|---|---|---|---|---|
| Decay Transition | Daughter level | Decay Type | $Q_n$ (keV) | $R_1$ (fm)<br>$R_2$ (fm)<br>$R_3$ (fm) | Log $f_0$ (Log $f_1)_{R_1}$<br>Log $f_0$ (Log $f_1)_{R_2}$<br>Log $f_0$ (Log $f_1)_{R_3}$ | Log $f_0t$(Log $f_1t)_{R_1}$<br>Log $f_0t$(Log $f_1t)_{R_2}$<br>Log $f_0t$(Log $f_1t)_{R_3}$ | Takahashi | NNDC |
| 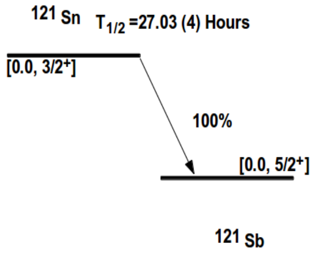 | $\left[0.0, \frac{5}{2}^+\right]$ | (a) | 390.600 | 5.935<br>4.680<br>5.364 | 0.0591<br>0.0730<br>0.0634 | 5.047<br>5.061<br>5.052 | - | 5.037 |
| 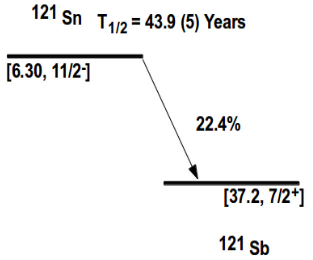 | $\left[37.2, \frac{7}{2}^+\right]$ | (u) | 359.700 | 5.935<br>4.680<br>5.364 | -0.1877<br>-0.1783<br>-0.1848 | 9.603<br>9.613<br>9.606 | - | 9.58 |
| 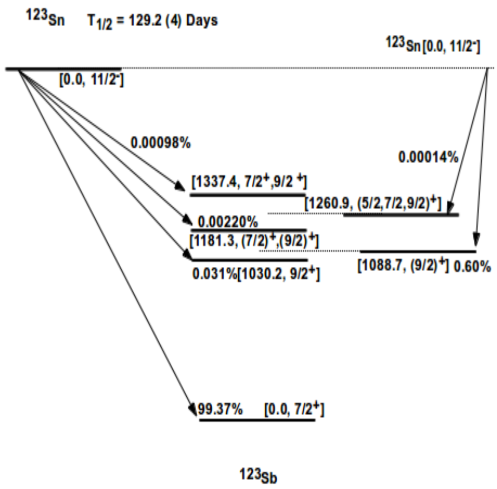 | $\left[0.0, \frac{7}{2}^+\right]$ | (u) | 1403.600 | 5.968<br>4.688<br>5.396 | 2.8398<br>2.8504<br>2.8431 | 9.890<br>9.901<br>9.894 | - | 9.876 |
| | $\left[1030.2, \frac{9}{2}^+\right]$ | (nu) | 373.400 | 5.968<br>4.688<br>5.396 | -0.0045<br>0.0094<br>-0.0002 | 10.552<br>10.566<br>10.556 | - | 10.54 |
| | $\left[1088.7, \left(\frac{9}{2}\right)^+\right]$ | (nu) | 314.900 | 5.968<br>4.688<br>5.396 | -0.2488<br>-0.2349<br>-0.2445 | 9.020<br>9.035<br>9.025 | - | 9.01 |
| | $\left[1181.3, \left(\frac{9}{2}\right)^+\right]$ | (nu) | 222.300 | 5.968<br>4.688<br>5.396 | -0.7360<br>-0.7221<br>-0.7317 | 10.969<br>10.983<br>10.974 | - | 10.96 |
| | $\left[1181.3, \left(\frac{7}{2}\right)^+\right]$ | (u) | 222.300 | 5.968<br>4.688<br>5.396 | -1.1233<br>-1.1146<br>-1.1206 | 10.582<br>10.591<br>10.585 | - | 10.96 |
| | $\left[[1260.9, \left(\frac{9}{2}\right)^+\right]$ | (nu) | 142.700 | 5.968<br>4.688<br>5.396 | -1.3441<br>-1.3302<br>-1.3398 | 11.558<br>11.572<br>11.562 | - | 11.55 |
| | $\left[1260.9, \left(\frac{7}{2}\right)^+\right]$ | (u) | 142.700 | 5.968<br>4.688<br>5.396 | -1.9211<br>-1.9131<br>-1.9186 | 10.981<br>10.989<br>10.983 | - | 11.55 |
| | $\left[1337.4, \frac{9}{2}^+\right]$ | (nu) | 66.200 | 5.968<br>4.688<br>5.396 | -2.3670<br>-2.3530<br>-2.3627 | 9.690<br>9.704<br>9.694 | - | 9.67 |
| | $\left[1337.4, \frac{7}{2}^+\right]$ | (u) | 66.200 | 5.968<br>4.688<br>5.396 | -3.1613<br>-3.1541<br>-3.1591 | 8.895<br>8.902<br>8.897 | - | 9.67 |

Table 1: (Cotnd.)

| Transition Details | | | | Present Calculation | | | Previous values | |
|---|---|---|---|---|---|---|---|---|
| Decay Transition | Daughter level | Decay Type | $Q_n$ (keV) | $R_1$<br>$R_2$<br>$R_3$ | Log $f_0$ (Log $f_1)_{R_1}$<br>Log $f_0$ (Log $f_1)_{R_2}$<br>Log $f_0$ (Log $f_1)_{R_3}$ | Log $f_0t$(Log $f_1t)_{R_1}$<br>Log $f_0t$(Log $f_1t)_{R_2}$<br>Log $f_0t$(Log $f_1t)_{R_3}$ | Takahashi | NNDC |
| 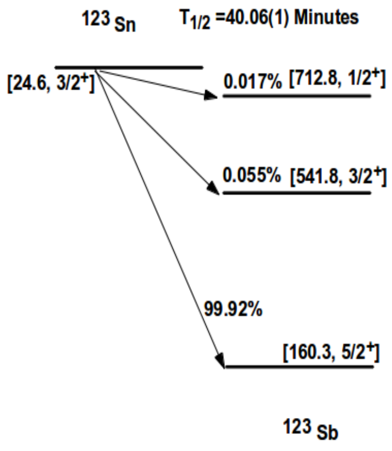 | $\left[160.3, \frac{5}{2}^+\right]$ | (a) | 1267.900 | 5.968<br>4.688<br>5.396 | 1.8714<br>1.8853<br>1.8757 | 5.253<br>5.266<br>5.257 | - | 5.241 |
| | $\left[541.8, \frac{3}{2}^+\right]$ | (a) | 886.400 | 5.968<br>4.688<br>5.396 | 1.2937<br>1.3077<br>1.2981 | 7.934<br>7.948<br>7.939 | - | 7.92 |
| | $\left[712.8, \frac{1}{2}^+\right]$ | (a) | 715.400 | 5.968<br>4.688<br>5.396 | 0.9597<br>0.9736<br>0.9640 | 8.110<br>8.124<br>8.114 | - | 8.10 |
| 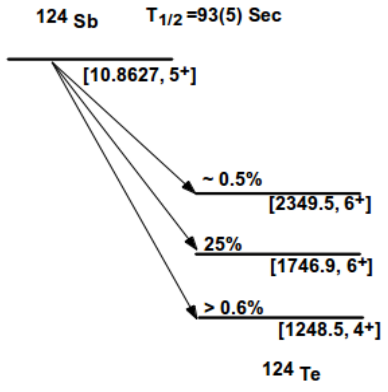 | $[1248.5, 4^+]$ | (a) | 1666.663 | 5.984<br>4.718<br>5.411 | 2.3498<br>2.3643<br>2.3543 | 6.540<br>6.555<br>6.545 | - | >6.2 |
| | $[1746.9, 6^+]$ | (a) | 1168.263 | 5.984<br>4.718<br>5.411 | 1.7554<br>1.7699<br>1.7598 | 4.326<br>4.340<br>4.330 | - | 4.3 |
| | $[2349.5, 6^+]$ | (a) | 565.663 | 5.984<br>4.718<br>5.411 | 0.6236<br>0.6381<br>0.6280 | 4.893<br>4.908<br>4.898 | - | $\sim$ 4.9 |
| 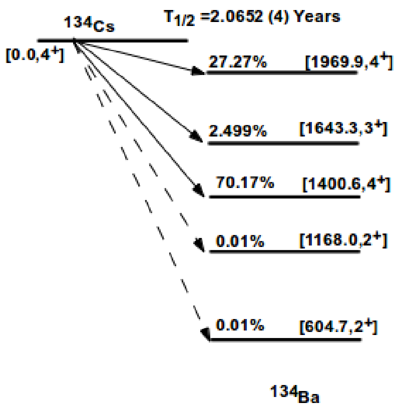 | $[1400.6, 4^+]$ | (a) | 658.100 | 6.141<br>4.832<br>5.563 | 0.9271<br>0.9428<br>0.9372 | 8.896<br>8.910<br>8.905 | - | 8.8849 |
| | $[1643.3, 3^+]$ | (a) | 415.400 | 6.141<br>4.832<br>5.563 | 0.2471<br>0.2628<br>0.2572 | 9.663<br>9.678<br>9.673 | - | 9.6528 |
| | $[1969.9, 4^+]$ | (a) | 88.800 | 6.141<br>4.832<br>5.563 | -1.8919<br>-1.8761<br>-1.8817 | 6.486<br>6.502<br>6.496 | - | 6.49 |

Table 1: (Cotnd.)

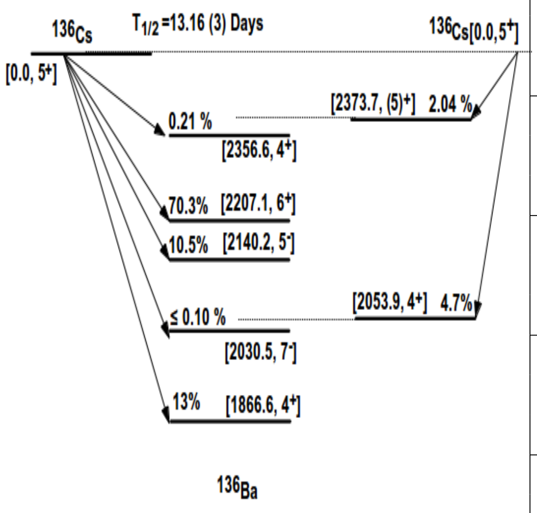


| Transition Details | | | | Present Calculation | | | Previous values | |
|---|---|---|---|---|---|---|---|---|
| Decay Transition | Daughter level | Decay Type | $Q_n$ (keV) | $R_1$ $R_2$ $R_3$ | Log $f_0$ (Log $f_1$)$_{R_1}$ Log $f_0$ (Log $f_1$)$_{R_2}$ Log $f_0$ (Log $f_1$)$_{R_3}$ | Log $f_0t$(Log $f_1t$)$_{R_1}$ Log $f_0t$(Log $f_1t$)$_{R_2}$ Log $f_0t$(Log $f_1t$)$_{R_3}$ | Takahashi | NNDC |
| | $[1866.6, 4^+]$ | (a) | 681.600 | 6.171 | 0.9803 | 7.922 | - | 7.91 |
| | | | | 4.833 | 0.9960 | 7.938 | | |
| | | | | 5.592 | 0.9904 | 7.932 | | |
| | $[2030.5, 7^-]$ | (u) | 517.700 | 6.171 | 0.6625 | 9.718 | - | ≥9.4 |
| | | | | 4.833 | 0.6737 | 9.729 | | |
| | | | | 5.592 | 0.6697 | 9.725 | | |
| | $[2053.9, 4^+]$ | (a) | 494.300 | 6.171 | 0.4997 | 7.883 | - | 7.87 |
| | | | | 4.833 | 0.5155 | 7.899 | | |
| | | | | 5.592 | 0.5099 | 7.894 | | |
| | $[2140.2, 5^-]$ | (nu) | 408.000 | 6.171 | 0.2202 | 7.255 | - | 7.25 |
| | | | | 4.833 | 0.2359 | 7.271 | | |
| | | | | 5.592 | 0.2303 | 7.265 | | |
| | $[2207.1, 6^+]$ | (a) | 341.100 | 6.171 | -0.0345 | 6.174 | - | 6.163 |
| | | | | 4.833 | -0.0187 | 6.190 | | |
| | | | | 5.592 | -0.0243 | 6.184 | | |
| | $[2356.6, 4^+]$ | (a) | 191.600 | 6.171 | -0.8395 | 7.894 | - | 7.88 |
| | | | | 4.833 | -0.8237 | 7.910 | | |
| | | | | 5.592 | -0.8293 | 7.904 | | |
| | $[2373.7, (5)^+]$ | (a) | 174.500 | 6.171 | -0.9695 | 6.777 | - | 6.768 |
| | | | | 4.833 | -0.9537 | 6.792 | | |
| | | | | 5.592 | -0.9593 | 6.787 | | |

Table 1: (Cotnd.)

| Transition Details | | | | Present Calculation | | | Previous values | |
|---|---|---|---|---|---|---|---|---|
| Decay Transition | Daughter level | Decay Type | $Q_n$ (keV) | $R_1$<br>$R_2$<br>$R_3$ | Log $f_0$ (Log $f_1)_{R_1}$<br>Log $f_0$ (Log $f_1)_{R_2}$<br>Log $f_0$ (Log $f_1)_{R_3}$ | Log $f_0t$(Log $f_1t)_{R_1}$<br>Log $f_0t$(Log $f_1t)_{R_2}$<br>Log $f_0t$(Log $f_1t)_{R_3}$ | Takahashi | NNDC |
| 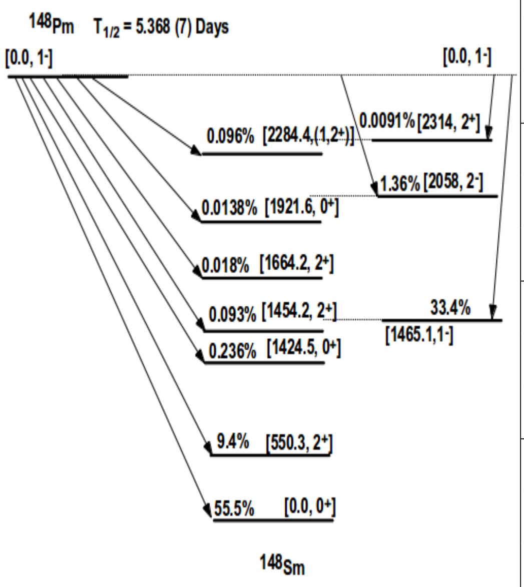 | $[0.0, 0^+]$ | (nu) | 2471.000 | 6.347<br>5.004<br>5.762 | 3.2109<br>3.2305<br>3.2170 | 9.133<br>9.153<br>9.139 | - | 9.117 |
| | $[550.3, 2^+]$ | (nu) | 1920.700 | 6.347<br>5.004<br>5.762 | 2.7716<br>2.7911<br>2.7776 | 9.467<br>9.484<br>9.471 | - | 9.450 |
| | $[1424.5, 0^+]$ | (nu) | 1046.500 | 6.347<br>5.004<br>5.762 | 1.7677<br>1.7872<br>1.7737 | 10.061<br>10.080<br>10.067 | - | 10.048 |
| | $[1454.2, 2^+]$ | (nu) | 1016.800 | 6.347<br>5.004<br>5.762 | 1.7219<br>1.7414<br>1.7280 | 10.420<br>10.439<br>10.426 | - | 10.406 |
| | $[1465.1, 1^-]$ | (a) | 1005.900 | 6.347<br>5.004<br>5.762 | 1.7045<br>1.7240<br>1.7105 | 7.848<br>7.867<br>7.854 | - | 7.834 |
| | $[1664.2, 2^+]$ | (nu) | 806.800 | 6.347<br>5.004<br>5.762 | 1.3607<br>1.3802<br>1.3668 | 10.772<br>10.791<br>10.778 | - | 10.76 |
| | $[1921.6, 0^+]$ | (nu) | 549.400 | 6.347<br>5.004<br>5.762 | 0.7812<br>0.8007<br>0.7872 | 10.307<br>10.327<br>10.313 | - | 10.29 |
| | $[2058, 2^-]$ | (a) | 413.000 | 6.347<br>5.004<br>5.762 | 0.3652<br>0.3848<br>0.3713 | 7.898<br>7.918<br>7.904 | - | 7.885 |
| | $[2284.4, (1, 2^+)]$ | (nu) | 186.600 | 6.347<br>5.004<br>5.762 | -0.7461<br>-0.7265<br>-0.7400 | 7.902<br>7.921<br>7.908 | - | 7.92 |
| | $[2314.0, 2^+]$ | (nu) | 157.000 | 6.347<br>5.004<br>5.762 | -0.9817<br>-0.9621<br>-0.9756 | 8.725<br>8.745<br>8.731 | - | 8.71 |

Table 1: (Cotnd.)

| Transition Details | | | | Present Calculation | | | Previous values | |
|---|---|---|---|---|---|---|---|---|
| Decay Transition | Daughter level | Decay Type | $Q_n$ (keV) | $R_1$<br>$R_2$<br>$R_3$ | Log $f_0$ (Log $f_1$)$_{R_1}$<br>Log $f_0$ (Log $f_1$)$_{R_2}$<br>Log $f_0$ (Log $f_1$)$_{R_3}$ | Log $f_0t$(Log $f_1t$)$_{R_1}$<br>Log $f_0t$(Log $f_1t$)$_{R_2}$<br>Log $f_0t$(Log $f_1t$)$_{R_3}$ | Takahashi | NNDC |
| 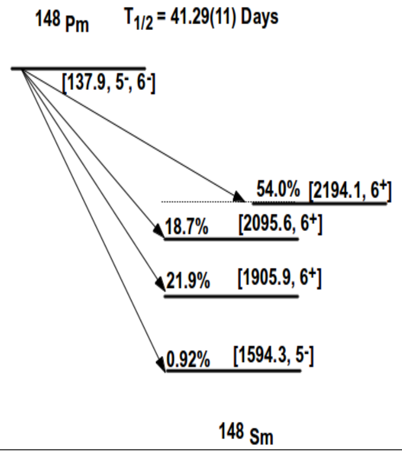  | $[1594.3, 5^-]$ | (a) | 1014.600 | 6.347<br>5.004<br>5.762 | 1.7189<br>1.7384<br>1.7249 | 10.307<br>10.327<br>10.314 | - | 10.29 |
| | $[1905.9, 6^+]$ | (nu) | 703.000 | 6.347<br>5.004<br>5.762 | 1.1505<br>1.1700<br>1.1565 | 8.362<br>8.382<br>8.368 | - | 8.348 |
| | $[2095.6, 6^+]$ | (nu) | 513.300 | 6.347<br>5.004<br>5.762 | 0.6821<br>0.7016<br>0.6881 | 7.963<br>7.982<br>7.969 | - | 7.949 |
| | $[2194.1, 6^+]$ | (nu) | 414.800 | 6.347<br>5.004<br>5.762 | 0.3723<br>0.3919<br>0.3784 | 7.192<br>7.212<br>7.198 | - | 7.178 |
| 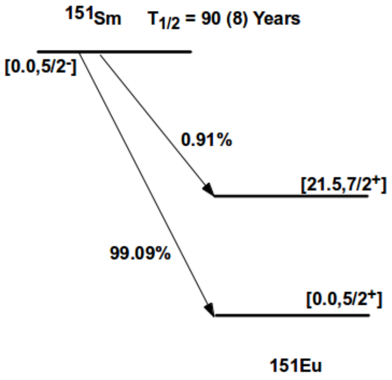  | $\left[0.0, \frac{5}{2}^+\right]$ | (nu) | 76.600 | 6.390<br>5.052<br>5.803 | -1.9259<br>-1.8998<br>-1.9137 | 7.531<br>7.557<br>7.543 | 7.53 | 7.51 |
| | $\left[21.5, \frac{7}{2}^+\right]$ | (nu) | 55.100 | 6.390<br>5.052<br>5.803 | -2.3613<br>-2.3352<br>-2.3491 | 9.133<br>9.159<br>9.145 | 9.13 | 9.11 |
| 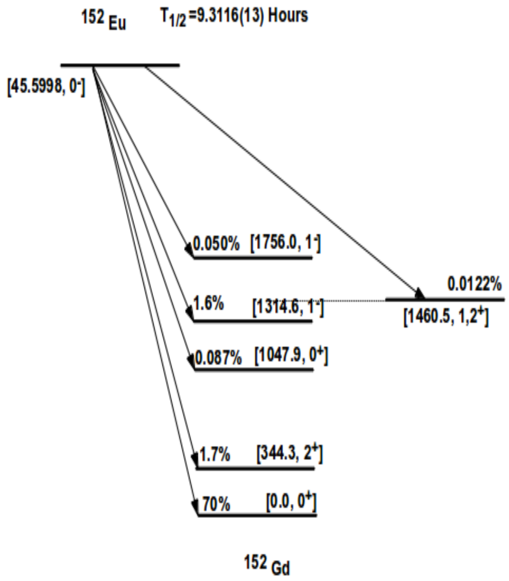  | $[0.0, 0^+]$ | (nu) | 1864.500 | 6.404<br>5.077<br>5.817 | 2.7528<br>2.7798<br>2.7654 | 7.433<br>7.460<br>7.455 | - | 7.42 |
| | $[344.3, 2^+]$ | (u) | 1520.200 | 6.404<br>5.077<br>5.817 | 3.2586<br>3.2795<br>3.2683 | 9.554<br>9.574<br>9.563 | - | 9.55 |
| | $[1047.9, 0^+]$ | (nu) | 816.600 | 6.404<br>5.077<br>5.817 | 1.4148<br>1.4418<br>1.4274 | 9.001<br>9.028<br>9.013 | - | 8.84 |
| | $[1314.6, 1^-]$ | (a) | 549.900 | 6.404<br>5.077<br>5.817 | 0.8194<br>0.8464<br>0.8320 | 7.141<br>7.168<br>7.153 | - | 7.13 |
| | $[1460.5, 1]$ | (nu) / (a) | 404.000 | 6.404<br>5.077<br>5.817 | 0.3722<br>0.3992<br>0.3848 | 8.811<br>8.838<br>8.824 | - | 8.80 |
| | $[1460.5, 2^+]$ | (u) | 404.000 | 6.404<br>5.077<br>5.817 | 0.3103<br>0.3287<br>0.3189 | 8.749<br>8.768<br>8.758 | - | 8.80 |
| | $[1756.0, 1^-]$ | (a) | 108.500 | 6.404<br>5.077<br>5.817 | -1.4420<br>-1.4150<br>-1.4294 | 6.384<br>6.411<br>6.397 | - | 6.39 |

Table 1: (Cotnd.)

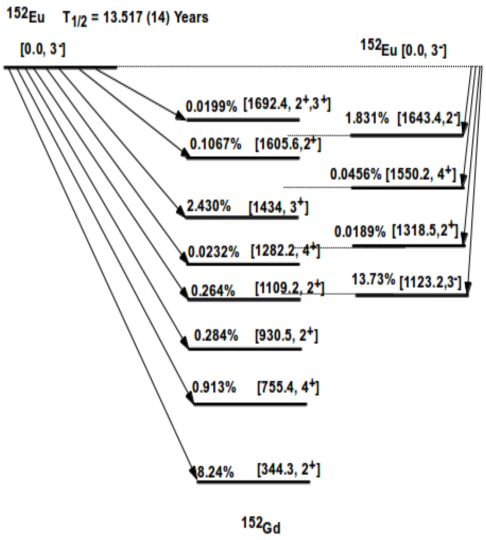


| Transition Details | | | | Present Calculation | | | Previous values | |
|---|---|---|---|---|---|---|---|---|
| Decay Transition | Daughter level | Decay Type | $Q_n$ (keV) | $R_1$ $R_2$ $R_3$ | Log $f_0$ (Log $f_1$)$_{R_1}$ Log $f_0$ (Log $f_1$)$_{R_2}$ Log $f_0$ (Log $f_1$)$_{R_3}$ | Log $f_0t$(Log $f_1t$)$_{R_1}$ Log $f_0t$(Log $f_1t$)$_{R_2}$ Log $f_0t$(Log $f_1t$)$_{R_3}$ | Takahashi | NNDC |
| | $[344.3, 2^+]$ | (nu) | 1474.600 | 6.404 | 2.3584 | 12.072 | - | 12.06 |
| | | | | 5.077 | 2.3854 | 12.099 | | |
| | | | | 5.817 | 2.3710 | 12.085 | | |
| | $[755.4, 4^+]$ | (nu) | 1063.500 | 6.404 | 1.8278 | 12.497 | - | 12.49 |
| | | | | 5.077 | 1.8548 | 12.524 | | |
| | | | | 5.817 | 1.8404 | 12.509 | | |
| | $[930.5, 2^+]$ | (nu) | 888.400 | 6.404 | 1.5456 | 12.722 | - | 12.71 |
| | | | | 5.077 | 1.5726 | 12.749 | | |
| | | | | 5.817 | 1.5588 | 12.735 | | |
| | $[1109.2, 2^+]$ | (nu) | 709.700 | 6.404 | 1.2009 | 12.409 | - | 12.40 |
| | | | | 5.077 | 1.2278 | 12.436 | | |
| | | | | 5.817 | 1.2134 | 12.421 | | |
| | $[1123.2, 3^-]$ | (a) | 695.700 | 6.404 | 1.1701 | 10.662 | - | 10.654 |
| | | | | 5.077 | 1.1970 | 10.689 | | |
| | | | | 5.817 | 1.1826 | 10.675 | | |
| | $[1282.2, 4^+]$ | (nu) | 536.700 | 6.404 | 0.7834 | 13.047 | - | 13.04 |
| | | | | 5.077 | 0.8104 | 13.074 | | |
| | | | | 5.817 | 0.7960 | 13.060 | | |
| | $[1318.5, 2^+]$ | (nu) | 500.400 | 6.404 | 0.6808 | 13.034 | - | 13.03 |
| | | | | 5.077 | 0.7077 | 13.061 | | |
| | | | | 5.817 | 0.6933 | 13.046 | | |
| | $[1434, 3^+]$ | (nu) | 384.900 | 6.404 | 0.3018 | 10.546 | - | 10.537 |
| | | | | 5.077 | 0.3288 | 10.573 | | |
| | | | | 5.817 | 0.3144 | 10.558 | | |
| | $[1550.2, 4^+]$ | (nu) | 268.700 | 6.404 | -0.2039 | 11.767 | - | 11.76 |
| | | | | 5.077 | -0.1769 | 11.794 | | |
| | | | | 5.817 | -0.1913 | 11.780 | | |
| | $[1605.6, 2^+]$ | (nu) | 213.300 | 6.404 | -0.5251 | 11.077 | - | 11.07 |
| | | | | 5.077 | -0.4981 | 11.104 | | |
| | | | | 5.817 | -0.5125 | 11.090 | | |
| | $[1643.4, 2^-]$ | (a) | 175.500 | 6.404 | -0.7923 | 9.575 | - | 9.567 |
| | | | | 5.077 | -0.7653 | 9.602 | | |
| | | | | 5.817 | -0.7797 | 9.587 | | |
| | $[1692.4, 2^+, 3^+]$ | (nu) | 126.500 | 6.404 | -1.2313 | 11.100 | - | 11.09 |
| | | | | 5.077 | -1.2043 | 11.127 | | |
| | | | | 5.817 | -1.2187 | 11.112 | | |

Table 1: (Cotnd.)

| Transition Details | | | | Present Calculation | | | Previous values | |
|---|---|---|---|---|---|---|---|---|
| Decay Transition | Daughter level | Decay Type | $Q_n$ (keV) | $R_1$<br>$R_2$<br>$R_3$ | Log $f_0$ (Log $f_1)_{R_1}$<br>Log $f_0$ (Log $f_1)_{R_2}$<br>Log $f_0$ (Log $f_1)_{R_3}$ | Log $f_0t$(Log $f_1t)_{R_1}$<br>Log $f_0t$(Log $f_1t)_{R_2}$<br>Log $f_0t$(Log $f_1t)_{R_3}$ | Takahashi | NNDC |
| 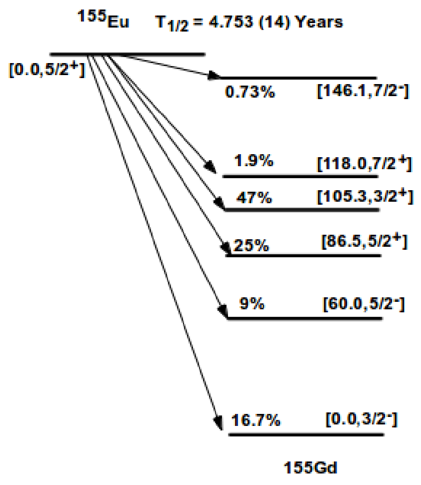 | $\left[0.0, \frac{3}{2}^-\right]$ | (nu) | 252.700 | 6.446<br>5.132<br>5.857 | -0.2883<br>-0.2613<br>-0.2757 | 8.665<br>8.692<br>8.677 | 8.78 | 8.65 |
| | $\left[60.0, \frac{5}{2}^-\right]$ | (nu) | 192.700 | 6.446<br>5.132<br>5.857 | -0.6633<br>-0.6363<br>-0.6507 | 8.558<br>8.585<br>8.571 | 8.57 | 8.54 |
| | $\left[86.5, \frac{5}{2}^+\right]$ | (a) | 166.200 | 6.446<br>5.132<br>5.857 | -0.8657<br>-0.8387<br>-0.8531 | 7.912<br>7.939<br>7.925 | 7.91 | 7.9 |
| | $\left[105.3, \frac{3}{2}^+\right]$ | (a) | 147.400 | 6.446<br>5.132<br>5.857 | -1.0296<br>-1.0026<br>-1.0170 | 7.474<br>7.501<br>7.487 | 7.47 | 7.46 |
| | $\left[118.0, \frac{7}{2}^+\right]$ | (a) | 134.700 | 6.446<br>5.132<br>5.857 | -1.1471<br>-1.1201<br>-1.1345 | 8.750<br>8.777<br>8.763 | 8.73 | 8.73 |
| | $\left[146.1, \frac{7}{2}^-\right]$ | (nu) | 106.600 | 6.446<br>5.132<br>5.857 | -1.4610<br>-1.4341<br>-1.4485 | 8.851<br>8.878<br>8.864 | 8.94 | 8.83 |
| 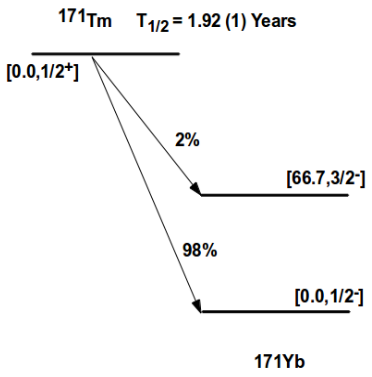 | $\left[0.0, \frac{1}{2}^-\right]$ | (nu) | 96.400 | 6.661<br>5.291<br>6.064 | -1.4581<br>-1.4344<br>-1.4507 | 6.333<br>6.356<br>6.340 | 6.32 | 6.3 |
| | $\left[66.7, \frac{3}{2}^-\right]$ | (nu) | 29.700 | 6.661<br>5.291<br>6.064 | -3.0196<br>-2.9959<br>-3.0122 | 6.461<br>6.485<br>6.469 | 6.45 | 6.5 |
| 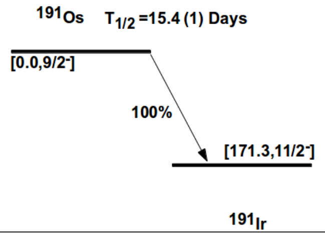 | $\left[171.3, \frac{11}{2}^-\right]$ | (a) | 141.400 | 6.911<br>5.397<br>6.304 | -0.7857<br>-0.7479<br>-0.7680 | 5.338<br>5.376<br>5.356 | 5.32 | 5.325 |

Table 1: (Cotnd.)

<table>
<tr><th colspan="4">Transition Details</th><th colspan="3">Present Calculation</th><th colspan="2">Previous values</th></tr>
<tr><th>Decay Transition</th><th>Daughter level</th><th>Decay Type</th><th>$Q_n$ (keV)</th><th>$R_1$<br>$R_2$<br>$R_3$</th><th>Log $f_0$ (Log $f_1)_{R_1}$<br>Log $f_0$ (Log $f_1)_{R_2}$<br>Log $f_0$ (Log $f_1)_{R_3}$</th><th>Log $f_0t$(Log $f_1t)_{R_1}$<br>Log $f_0t$(Log $f_1t)_{R_2}$<br>Log $f_0t$(Log $f_1t)_{R_3}$</th><th>Takahashi</th><th>NNDC</th></tr>
<tr><td rowspan="3">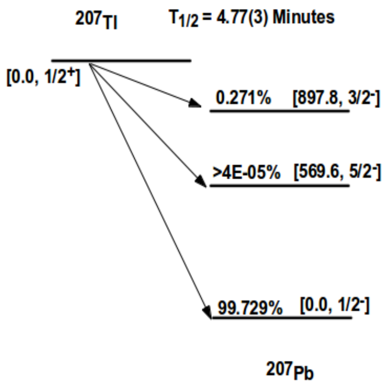
</td><td>$\left[0.0, \frac{1}{2}^-\right]$</td><td>(nu)</td><td>1418.000</td><td>7.099<br>5.494<br>6.484</td><td>2.6681<br>2.7115<br>2.6780</td><td>5.126<br>5.170<br>5.136</td><td>-</td><td>5.108</td></tr>
<tr><td>$\left[569.6, \frac{5}{2}^-\right]$</td><td>(u)</td><td>848.800</td><td>7.099<br>5.494<br>6.484</td><td>2.2681<br>2.3013<br>2.2756</td><td>11.123<br>11.156<br>11.131</td><td>-</td><td>>10.5</td></tr>
<tr><td>$\left[897.8, \frac{3}{2}^-\right]$</td><td>(nu)</td><td>520.200</td><td>7.099<br>5.494<br>6.484</td><td>1.1450<br>1.1884<br>1.1549</td><td>6.169<br>6.212<br>6.179</td><td>-</td><td>6.157</td></tr>
<tr><td rowspan="2">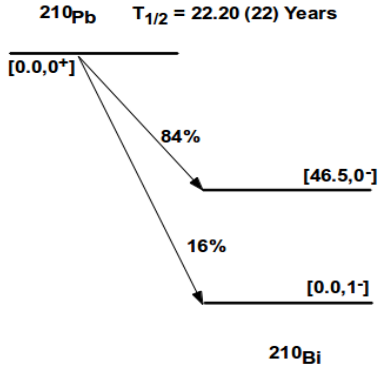
</td><td>$[0.0, 1^-]$</td><td>(nu)</td><td>63.500</td><td>7.133<br>5.530<br>6.517</td><td>-1.7061<br>-1.6615<br>-1.6959</td><td>7.935<br>7.980<br>7.945</td><td>7.84</td><td>7.9</td></tr>
<tr><td>$[46.5, 0^-]$</td><td>(nu)</td><td>17.000</td><td>7.133<br>5.530<br>6.517</td><td>-3.4454<br>-3.4008<br>-3.4353</td><td>5.476<br>5.520<br>5.486</td><td>5.46</td><td>5.4</td></tr>
<tr><td rowspan="4">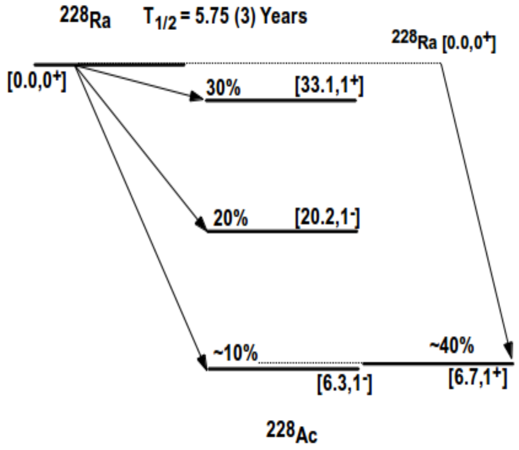
</td><td>$[6.3, 1^-]$</td><td>(nu)</td><td>39.500</td><td>7.331<br>-<br>6.707</td><td>-2.1848<br>-<br>-2.1616</td><td>7.074<br>-<br>7.097</td><td>-</td><td>$\sim$ 7.1</td></tr>
<tr><td>$[6.7, 1^+]$</td><td>(a)</td><td>39.100</td><td>7.331<br>-<br>6.707</td><td>-2.1848<br>-<br>-2.1616</td><td>6.472<br>-<br>6.495</td><td>(6.5)</td><td>$\sim$ 6.5</td></tr>
<tr><td>$[20.2, 1^-]$</td><td>(nu)</td><td>25.600</td><td>7.331<br>-<br>6.707</td><td>-2.7515<br>-<br>-2.7284</td><td>6.206<br>-<br>6.229</td><td>-</td><td>6.20</td></tr>
<tr><td>$[33.1, 1^+]$</td><td>(a)</td><td>12.700</td><td>7.331<br>-<br>6.707</td><td>-3.6585<br>-<br>-3.6353</td><td>5.123<br>-<br>5.146</td><td>(5.0)</td><td>5.12</td></tr>
</table>

Table 1: (Cotnd.)

| Transition Details | | | | Present Calculation | | | Previous values | |
|---|---|---|---|---|---|---|---|---|
| Decay Transition | Daughter level | Decay Type | $Q_n$ (keV) | $R_1$<br>$R_2$<br>$R_3$ | Log $f_0$ (Log $f_1)_{R_1}$<br>Log $f_0$ (Log $f_1)_{R_2}$<br>Log $f_0$ (Log $f_1)_{R_3}$ | Log $f_0t$(Log $f_1t)_{R_1}$<br>Log $f_0t$(Log $f_1t)_{R_2}$<br>Log $f_0t$(Log $f_1t)_{R_3}$ | Takahashi | NNDC |
| 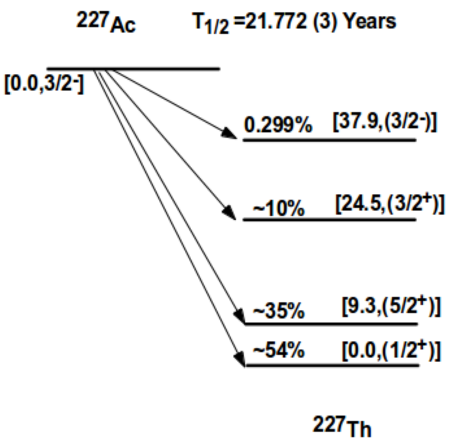 | $\left[0.0, \left(\frac{1}{2}^+\right)\right]$ | (nu) | 44.800 | 7.320<br>5.740<br>6.696 | -1.9817<br>-1.9311<br>-1.9579 | 7.123<br>7.173<br>7.146 | 7.09 | ∼ 7.1 |
| | $\left[9.3, \left(\frac{5}{2}^+\right)\right]$ | (nu) | 35.500 | 7.320<br>5.740<br>6.696 | -2.3015<br>-2.2509<br>-2.2777 | 6.991<br>7.042<br>7.015 | 6.97 | ∼ 7.0 |
| | $\left[24.5, \left(\frac{3}{2}^+\right)\right]$ | (nu) | 20.300 | 7.320<br>5.740<br>6.696 | -3.0163<br>-2.9658<br>-2.9925 | 6.820<br>6.871<br>6.844 | 6.75 | ∼ 6.8 |
| | $\left[37.9, \left(\frac{3}{2}^-\right)\right]$ | (a) | 6.900 | 7.320<br>5.740<br>6.696 | -4.3881<br>-4.3376<br>-4.3643 | 6.972<br>7.022<br>6.995 | - | 6.9 |
| 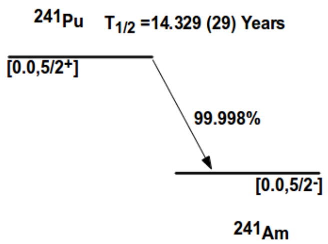 | $\left[0.0, \frac{5}{2}^-\right]$ | (nu) | 20.780 | 7.468<br>5.893<br>6.837 | -2.8419<br>-2.7846<br>-2.8288 | 5.813<br>5.870<br>5.826 | 5.79 | 5.788 |

Table 2: Bound and Continuum Decay rates for Bare Atom.

| Transition Details | Bound State Decay | | Continuum State Decay | | Bound to Continuum Ratio |
|---|---|---|---|---|---|
| | $\lambda_B$ for $R_1$ in $Sec^{-1}$<br>$\lambda_B$ for $R_2$ in $Sec^{-1}$<br>$\lambda_B$ for $R_3$ in $Sec^{-1}$ | Prev. Values<br>Takahashi | $\lambda_C$ for $R_1$ in $Sec^{-1}$<br>$\lambda_C$ for $R_2$ in $Sec^{-1}$<br>$\lambda_C$ for $R_3$ in $Sec^{-1}$ | Prev. Values<br>Takahashi | |
| $^{63}Ni \rightarrow ^{63}Cu$<br>$\left[0.0, \frac{1}{2}^-\right] \rightarrow \left[0.0, \frac{3}{2}^-\right]$ | $2.815 \times 10^{-10}$<br>$2.801 \times 10^{-10}$<br>$2.826 \times 10^{-10}$ | $3.0 \times 10^{-10}$ | $1.843 \times 10^{-10}$<br>$1.833 \times 10^{-10}$<br>$1.835 \times 10^{-10}$ | $1.9 \times 10^{-10}$ | $1.527 \times 10^{0}$<br>$1.528 \times 10^{0}$<br>$1.540 \times 10^{0}$ |
| $^{66}Ni \rightarrow ^{66}Cu$<br>$[0.0, 0^+] \rightarrow [0.0, 1^+]$ | $8.486 \times 10^{-7}$<br>-<br>$8.598 \times 10^{-7}$ | $1.0 \times 10^{-6}$ | $3.361 \times 10^{-6}$<br>-<br>$3.377 \times 10^{-6}$ | $3.4 \times 10^{-6}$ | $2.525 \times 10^{-1}$<br>-<br>$2.546 \times 10^{-1}$ |
| $^{85}Kr \rightarrow ^{85}Rb$<br>$\left[0.0, \frac{9}{2}^+\right] \rightarrow \left[0.0, \frac{5}{2}^-\right]$ | $1.844 \times 10^{-10}$<br>$1.851 \times 10^{-10}$<br>$1.848 \times 10^{-10}$ | - | $1.959 \times 10^{-9}$<br>$1.957 \times 10^{-9}$<br>$1.957 \times 10^{-9}$ | - | $9.413 \times 10^{-2}$<br>$9.458 \times 10^{-2}$<br>$9.443 \times 10^{-2}$ |
| $^{85}Kr \rightarrow ^{85}Rb$<br>$\left[0.0, \frac{9}{2}^+\right] \rightarrow \left[514.0, \frac{9}{2}^+\right]$ | $6.021 \times 10^{-12}$<br>$6.034 \times 10^{-12}$<br>$6.022 \times 10^{-12}$ | - | $8.002 \times 10^{-12}$<br>$8.000 \times 10^{-12}$<br>$7.995 \times 10^{-12}$ | - | $7.524 \times 10^{-1}$<br>$7.543 \times 10^{-1}$<br>$7.532 \times 10^{-1}$ |
| $^{85}Kr \rightarrow ^{85}Rb$<br>$\left[304.86, \frac{1}{2}^-\right] \rightarrow \left[151.2, \frac{3}{2}^-\right]$ | $2.334 \times 10^{-6}$<br>$2.334 \times 10^{-6}$<br>$2.335 \times 10^{-6}$ | - | $3.300 \times 10^{-5}$<br>$3.298 \times 10^{-5}$<br>$3.300 \times 10^{-5}$ | - | $7.073 \times 10^{-2}$<br>$7.077 \times 10^{-2}$<br>$7.076 \times 10^{-2}$ |
| $^{85}Kr \rightarrow ^{85}Rb$<br>$\left[304.86, \frac{1}{2}^-\right] \rightarrow \left[281.0, \frac{1}{2}^-\right]$ | $1.223 \times 10^{-8}$<br>$1.222 \times 10^{-8}$<br>$1.224 \times 10^{-8}$ | - | $1.303 \times 10^{-7}$<br>$1.302 \times 10^{-7}$<br>$1.303 \times 10^{-7}$ | - | $9.386 \times 10^{-2}$<br>$9.378 \times 10^{-2}$<br>$9.394 \times 10^{-2}$ |
| $^{85}Kr \rightarrow ^{85}Rb$<br>$\left[304.86, \frac{1}{2}^-\right] \rightarrow \left[731.9, \frac{3}{2}^-\right]$ | $3.252 \times 10^{-9}$<br>$3.251 \times 10^{-9}$<br>$3.254 \times 10^{-9}$ | - | $7.658 \times 10^{-9}$<br>$7.653 \times 10^{-9}$<br>$7.654 \times 10^{-9}$ | - | $4.247 \times 10^{-1}$<br>$4.248 \times 10^{-1}$<br>$4.251 \times 10^{-1}$ |
| $^{93}Zr \rightarrow ^{93}Nb$<br>$\left[0.0, \frac{5}{2}^+\right] \rightarrow \left[30.8, \frac{1}{2}^-\right]$ | $6.132 \times 10^{-15}$<br>$6.208 \times 10^{-15}$<br>$6.177 \times 10^{-15}$ | $1.3 \times 10^{-14}$ | $6.874 \times 10^{-15}$<br>$7.195 \times 10^{-15}$<br>$6.858 \times 10^{-15}$ | $1.1 \times 10^{-14}$ | $8.921 \times 10^{-1}$<br>$8.628 \times 10^{-1}$<br>$9.007 \times 10^{-1}$ |
| $^{95}Nb \rightarrow ^{95}Mo$<br>$\left[0.0, \frac{9}{2}^+\right] \rightarrow \left[765.8, \frac{7}{2}^+\right]$ | $2.296 \times 10^{-7}$<br>$2.296 \times 10^{-7}$<br>$2.312 \times 10^{-7}$ | $2.4 \times 10^{-7}$ | $2.032 \times 10^{-7}$<br>$2.039 \times 10^{-7}$<br>$2.018 \times 10^{-7}$ | $2.1 \times 10^{-7}$ | $1.130 \times 10^{0}$<br>$1.126 \times 10^{0}$<br>$1.146 \times 10^{0}$ |

Table 2: (Cotnd.)

| Transition Details | Bound State Decay: $\lambda_B$ for R$_1$ in Sec$^{-1}$, $\lambda_B$ for R$_2$ in Sec$^{-1}$, $\lambda_B$ for R$_3$ in Sec$^{-1}$ | Bound State Decay: Prev. Value Takahashi | Continuum State Decay: $\lambda_C$ for R$_1$ in Sec$^{-1}$, $\lambda_C$ for R$_2$ in Sec$^{-1}$, $\lambda_C$ for R$_3$ in Sec$^{-1}$ | Continuum State Decay: Prev. Value Takahashi | Bound to Continuum Ratio |
|---|---|---|---|---|---|
| $^{95}Nb\rightarrow^{95}Mo$ $\left[234.7, \frac{1}{2}^{-}\right] \rightarrow \left[0.0, \frac{5}{2}^{+}\right]$ | $4.203\times10^{-9}$<br>$4.222\times10^{-9}$<br>$4.230\times10^{-9}$ | - | $6.894\times10^{-8}$<br>$6.887\times10^{-8}$<br>$6.883\times10^{-8}$ | - | $6.097\times10^{-2}$<br>$6.130\times10^{-2}$<br>$6.146\times10^{-2}$ |
| $^{95}Nb\rightarrow^{95}Mo$ $\left[234.7, \frac{1}{2}^{-}\right] \rightarrow \left[204.1, \frac{3}{2}^{+}\right]$ | $3.922\times10^{-9}$<br>$3.921\times10^{-9}$<br>$3.945\times10^{-9}$ | - | $5.207\times10^{-8}$<br>$5.208\times10^{-8}$<br>$5.208\times10^{-8}$ | - | $7.532\times10^{-2}$<br>$7.529\times10^{-2}$<br>$7.575\times10^{-2}$ |
| $^{95}Nb\rightarrow^{95}Mo$ $\left[234.7, \frac{1}{2}^{-}\right] \rightarrow \left[786.2, \frac{1}{2}^{+}\right]$ | $5.024\times10^{-10}$<br>$5.011\times10^{-10}$<br>$5.045\times10^{-10}$ | - | $1.495\times10^{-9}$<br>$1.491\times10^{-9}$<br>$1.491\times10^{-9}$ | - | $3.361\times10^{-1}$<br>$3.360\times10^{-1}$<br>$3.384\times10^{-1}$ |
| $^{95}Nb\rightarrow^{95}Mo$ $\left[234.7, \frac{1}{2}^{-}\right] \rightarrow \left[820.6, \frac{3}{2}^{+}\right]$ | $2.991\times10^{-12}$<br>$2.998\times10^{-12}$<br>$3.010\times10^{-12}$ | - | $7.746\times10^{-12}$<br>$7.740\times10^{-12}$<br>$7.745\times10^{-12}$ | - | $3.861\times10^{-1}$<br>$3.873\times10^{-1}$<br>$3.886\times10^{-1}$ |
| $^{95}Nb\rightarrow^{95}Mo$ $\left[234.7, \frac{1}{2}^{-}\right] \rightarrow \left[1039.3, \frac{1}{2}^{+}\right]$ | $4.193\times10^{-13}$<br>$4.193\times10^{-13}$<br>$4.220\times10^{-13}$ | - | $2.482\times10^{-13}$<br>$2.426\times10^{-13}$<br>$2.465\times10^{-13}$ | - | $1.689\times10^{0}$<br>$1.728\times10^{0}$<br>$1.712\times10^{0}$ |
| $^{99}Tc\rightarrow^{99}Ru$ $\left[142.7, \frac{1}{2}^{-}\right] \rightarrow \left[0.0, \frac{5}{2}^{+}\right]$ | $7.189\times10^{-11}$<br>$7.257\times10^{-11}$<br>$7.225\times10^{-11}$ | - | $2.980\times10^{-10}$<br>$2.977\times10^{-10}$<br>$2.975\times10^{-10}$ | - | $2.412\times10^{-1}$<br>$2.438\times10^{-1}$<br>$2.429\times10^{-1}$ |
| $^{99}Tc\rightarrow^{99}Ru$ $\left[142.7, \frac{1}{2}^{-}\right] \rightarrow \left[89.6, \frac{3}{2}^{+}\right]$ | $3.204\times10^{-10}$<br>$3.211\times10^{-10}$<br>$3.219\times10^{-10}$ | - | $7.815\times10^{-10}$<br>$7.817\times10^{-10}$<br>$7.819\times10^{-10}$ | - | $4.100\times10^{-1}$<br>$4.108\times10^{-1}$<br>$4.117\times10^{-1}$ |
| $^{99}Tc\rightarrow^{99}Ru$ $\left[142.7, \frac{1}{2}^{-}\right] \rightarrow \left[322.4, \frac{3}{2}^{+}\right]$ | $5.965\times10^{-11}$<br>$5.995\times10^{-11}$<br>$5.995\times10^{-11}$ | - | $2.998\times10^{-11}$<br>$2.930\times10^{-11}$<br>$2.977\times10^{-11}$ | - | $1.990\times10^{0}$<br>$2.046\times10^{0}$<br>$2.014\times10^{0}$ |
| $^{106}Ru\rightarrow^{106}Rh$ $\left[0.0, 0^{+}\right] \rightarrow \left[0.0, 1^{+}\right]$ | $2.001\times10^{-7}$<br>-<br>$1.998\times10^{-7}$ | $2.1\times10^{-7}$ | $1.239\times10^{-8}$<br>-<br>$1.222\times10^{-8}$ | $1.2\times10^{-8}$ | $1.615\times10^{1}$<br>-<br>$1.635\times10^{1}$ |
| $^{107}Pd\rightarrow^{107}Ag$ $\left[0.0, \frac{5}{2}^{+}\right] \rightarrow \left[0.0, \frac{1}{2}^{-}\right]$ | $4.822\times10^{-15}$<br>$4.896\times10^{-15}$<br>$4.849\times10^{-15}$ | $8.2\times10^{-15}$ | $1.235\times10^{-15}$<br>$1.218\times10^{-15}$<br>$1.224\times10^{-15}$ | $1.8\times10^{-15}$ | $3.904\times10^{0}$<br>$4.020\times10^{0}$<br>$3.962\times10^{0}$ |

Table 2: (Cotnd.)

| Transition Details | Bound State Decay: $\lambda_B$ for $R_1$ in $Sec^{-1}$ / $\lambda_B$ for $R_2$ in $Sec^{-1}$ / $\lambda_B$ for $R_3$ in $Sec^{-1}$ | Bound State Decay: Prev. Value Takahashi | Continuum State Decay: $\lambda_C$ for $R_1$ in $Sec^{-1}$ / $\lambda_C$ for $R_2$ in $Sec^{-1}$ / $\lambda_C$ for $R_3$ in $Sec^{-1}$ | Continuum State Decay: Prev. Value Takahashi | Bound to Continuum Ratio |
|---|---|---|---|---|---|
| $^{110}Ag \rightarrow ^{110}Cd$ $[117.59, 6^+] \rightarrow [2479.9, 6^+]$ | $2.564 \times 10^{-9}$ $2.576 \times 10^{-9}$ $2.554 \times 10^{-9}$ | - | $9.589 \times 10^{-9}$ $9.597 \times 10^{-9}$ $9.587 \times 10^{-9}$ | - | $2.674 \times 10^{-1}$ $2.684 \times 10^{-1}$ $2.664 \times 10^{-1}$ |
| $^{110}Ag \rightarrow ^{110}Cd$ $[117.59, 6^+] \rightarrow [2539.7, 5^-]$ | $6.001 \times 10^{-12}$ $5.999 \times 10^{-12}$ $5.950 \times 10^{-12}$ | - | $1.861 \times 10^{-11}$ $1.853 \times 10^{-11}$ $1.852 \times 10^{-11}$ | - | $3.225 \times 10^{-1}$ $3.237 \times 10^{-1}$ $3.213 \times 10^{-1}$ |
| $^{110}Ag \rightarrow ^{110}Cd$ $[117.59, 6^+] \rightarrow [2659.9, 5^-]$ | $5.391 \times 10^{-12}$ $5.401 \times 10^{-12}$ $5.369 \times 10^{-12}$ | - | $1.075 \times 10^{-11}$ $1.074 \times 10^{-11}$ $1.075 \times 10^{-11}$ | - | $5.015 \times 10^{-1}$ $5.029 \times 10^{-1}$ $4.994 \times 10^{-1}$ |
| $^{110}Ag \rightarrow ^{110}Cd$ $[117.59, 6^+] \rightarrow [2842.6, (5)^-]$ | $9.517 \times 10^{-12}$ $9.557 \times 10^{-12}$ $9.478 \times 10^{-12}$ | - | $6.381 \times 10^{-12}$ $6.429 \times 10^{-12}$ $6.377 \times 10^{-12}$ | - | $1.491 \times 10^{0}$ $1.487 \times 10^{0}$ $1.486 \times 10^{0}$ |
| $^{110}Ag \rightarrow ^{110}Cd$ $[117.59, 6^+] \rightarrow [2876.8, 6^+]$ | $2.238 \times 10^{-10}$ $2.249 \times 10^{-10}$ $2.229 \times 10^{-10}$ | - | $1.079 \times 10^{-10}$ $1.050 \times 10^{-10}$ $1.059 \times 10^{-10}$ | - | $2.074 \times 10^{0}$ $2.142 \times 10^{0}$ $2.105 \times 10^{0}$ |
| $^{110}Ag \rightarrow ^{110}Cd$ $[117.59, 6^+] \rightarrow [2926.7, 5^+]$ | $7.537 \times 10^{-8}$ $7.550 \times 10^{-8}$ $7.507 \times 10^{-8}$ | $7.8 \times 10^{-8}$ | $1.643 \times 10^{-8}$ $1.640 \times 10^{-8}$ $1.642 \times 10^{-8}$ | $1.7 \times 10^{-8}$ | $4.587 \times 10^{0}$ $4.604 \times 10^{0}$ $4.572 \times 10^{0}$ |
| $^{113}Cd \rightarrow ^{113}In$ $\left[263.7, \frac{11}{2}^-\right] \rightarrow \left[0.0, \frac{9}{2}^+\right]$ | $3.572 \times 10^{-10}$ $3.583 \times 10^{-10}$ $3.600 \times 10^{-10}$ | - | $1.490 \times 10^{-9}$ $1.489 \times 10^{-9}$ $1.490 \times 10^{-9}$ | - | $2.397 \times 10^{-1}$ $2.406 \times 10^{-1}$ $2.416 \times 10^{-1}$ |
| $^{115}Cd \rightarrow ^{115}In$ $\left[181.0, \frac{11}{2}^-\right] \rightarrow \left[0.0, \frac{9}{2}^+\right]$ | $6.724 \times 10^{-9}$ $6.781 \times 10^{-9}$ $6.775 \times 10^{-9}$ | - | $1.712 \times 10^{-7}$ $1.716 \times 10^{-7}$ $1.712 \times 10^{-7}$ | - | $3.928 \times 10^{-2}$ $3.952 \times 10^{-2}$ $3.957 \times 10^{-2}$ |
| $^{115}Cd \rightarrow ^{115}In$ $\left[181.0, \frac{11}{2}^-\right] \rightarrow \left[933.8, \frac{7}{2}^+\right]$ | $5.315 \times 10^{-10}$ $5.398 \times 10^{-10}$ $5.368 \times 10^{-10}$ | - | $2.890 \times 10^{-9}$ $2.893 \times 10^{-9}$ $2.890 \times 10^{-9}$ | - | $1.839 \times 10^{-1}$ $1.866 \times 10^{-1}$ $1.857 \times 10^{-1}$ |
| $^{115}Cd \rightarrow ^{115}In$ $\left[181.0, \frac{11}{2}^-\right] \rightarrow \left[1132.6, \frac{11}{2}^+\right]$ | $3.161 \times 10^{-11}$ $3.180 \times 10^{-11}$ $3.184 \times 10^{-11}$ | - | $1.025 \times 10^{-10}$ $1.025 \times 10^{-10}$ $1.025 \times 10^{-10}$ | - | $3.084 \times 10^{-1}$ $3.102 \times 10^{-1}$ $3.106 \times 10^{-1}$ |
| $^{115}Cd \rightarrow ^{115}In$ $\left[181.0, \frac{11}{2}^-\right] \rightarrow \left[1290.6, \frac{13}{2}^+\right]$ | $8.225 \times 10^{-10}$ $8.278 \times 10^{-10}$ $8.289 \times 10^{-10}$ | - | $1.495 \times 10^{-9}$ $1.496 \times 10^{-9}$ $1.496 \times 10^{-9}$ | - | $5.502 \times 10^{-1}$ $5.533 \times 10^{-1}$ $5.541 \times 10^{-1}$ |

Table 2: (Cotnd.)

| Transition Details | Bound State Decay: $\lambda_B$ for R$_1$ in Sec$^{-1}$ / $\lambda_B$ for R$_2$ in Sec$^{-1}$ / $\lambda_B$ for R$_3$ in Sec$^{-1}$ | Bound State Decay: Prev. Value Takahashi | Continuum State Decay: $\lambda_C$ for R$_1$ in Sec$^{-1}$ / $\lambda_C$ for R$_2$ in Sec$^{-1}$ / $\lambda_C$ for R$_3$ in Sec$^{-1}$ | Continuum State Decay: Prev. Value Takahashi | Bound to Continuum Ratio |
|---|---|---|---|---|---|
| $^{115}Cd \rightarrow ^{115}In$ $\left[181.0, \frac{11}{2}^-\right] \rightarrow \left[1418.3, \left(\frac{9}{2}\right)^+\right]$ | $5.269 \times 10^{-10}$<br>$5.303 \times 10^{-10}$<br>$5.311 \times 10^{-10}$ | - | $4.749 \times 10^{-10}$<br>$4.757 \times 10^{-10}$<br>$4.781 \times 10^{-10}$ | - | $1.109 \times 10^{0}$<br>$1.115 \times 10^{0}$<br>$1.111 \times 10^{0}$ |
| $^{115}Cd \rightarrow ^{115}In$ $\left[181.0, \frac{11}{2}^-\right] \rightarrow \left[1448.8, \frac{9}{2}^+\right]$ | $4.356 \times 10^{-11}$<br>$4.383 \times 10^{-11}$<br>$4.389 \times 10^{-11}$ | - | $3.159 \times 10^{-11}$<br>$3.147 \times 10^{-11}$<br>$3.130 \times 10^{-11}$ | - | $1.379 \times 10^{0}$<br>$1.393 \times 10^{0}$<br>$1.402 \times 10^{0}$ |
| $^{115}Cd \rightarrow ^{115}In$ $\left[181.0, \frac{11}{2}^-\right] \rightarrow \left[1486.1, \frac{9}{2}^+\right]$ | $2.097 \times 10^{-12}$<br>$2.110 \times 10^{-12}$<br>$2.113 \times 10^{-12}$ | - | $1.051 \times 10^{-12}$<br>$1.050 \times 10^{-12}$<br>$1.072 \times 10^{-12}$ | - | $1.995 \times 10^{0}$<br>$2.010 \times 10^{0}$<br>$1.971 \times 10^{0}$ |
| $^{121}Sn \rightarrow ^{121}Sb$ $\left[0.0, \frac{3}{2}^+\right] \rightarrow \left[0.0, \frac{5}{2}^+\right]$ | $3.243 \times 10^{-6}$<br>$3.261 \times 10^{-6}$<br>$3.258 \times 10^{-6}$ | - | $6.661 \times 10^{-6}$<br>$6.660 \times 10^{-6}$<br>$6.646 \times 10^{-6}$ | - | $4.869 \times 10^{-1}$<br>$4.935 \times 10^{-1}$<br>$4.902 \times 10^{-1}$ |
| $^{121}Sn \rightarrow ^{121}Sb$ $\left[6.30, \frac{11}{2}^-\right] \rightarrow \left[37.2, \frac{7}{2}^+\right]$ | $7.724 \times 10^{-11}$<br>$7.836 \times 10^{-11}$<br>$7.792 \times 10^{-11}$ | - | $1.404 \times 10^{-10}$<br>$1.417 \times 10^{-10}$<br>$1.408 \times 10^{-10}$ | - | $5.501 \times 10^{-1}$<br>$5.530 \times 10^{-1}$<br>$5.534 \times 10^{-1}$ |
| $^{123}Sn \rightarrow ^{123}Sb$ $\left[0.0, \frac{11}{2}^-\right] \rightarrow \left[0.0, \frac{7}{2}^+\right]$ | $4.314 \times 10^{-9}$<br>$4.367 \times 10^{-9}$<br>$4.342 \times 10^{-9}$ | - | $5.975 \times 10^{-8}$<br>$5.970 \times 10^{-8}$<br>$5.965 \times 10^{-8}$ | - | $7.220 \times 10^{-2}$<br>$7.315 \times 10^{-2}$<br>$7.279 \times 10^{-2}$ |
| $^{123}Sn \rightarrow ^{123}Sb$ $\left[0.0, \frac{11}{2}^-\right] \rightarrow \left[1030.2, \frac{9}{2}^+\right]$ | $9.320 \times 10^{-12}$<br>$9.368 \times 10^{-12}$<br>$9.377 \times 10^{-12}$ | - | $1.793 \times 10^{-11}$<br>$1.792 \times 10^{-11}$<br>$1.793 \times 10^{-11}$ | - | $5.198 \times 10^{-1}$<br>$5.228 \times 10^{-1}$<br>$5.230 \times 10^{-1}$ |
| $^{123}Sn \rightarrow ^{123}Sb$ $\left[0.0, \frac{11}{2}^-\right] \rightarrow \left[1088.7, \left(\frac{9}{2}\right)^+\right]$ | $2.307 \times 10^{-10}$<br>$2.313 \times 10^{-10}$<br>$2.316 \times 10^{-10}$ | - | $3.435 \times 10^{-10}$<br>$3.427 \times 10^{-10}$<br>$3.428 \times 10^{-10}$ | - | $6.716 \times 10^{-1}$<br>$6.749 \times 10^{-1}$<br>$6.756 \times 10^{-1}$ |
| $^{123}Sn \rightarrow ^{123}Sb$ $\left[0.0, \frac{11}{2}^-\right] \rightarrow \left[1181.3, \left(\frac{9}{2}\right)^+\right]$ | $1.369 \times 10^{-12}$<br>$1.377 \times 10^{-12}$<br>$1.375 \times 10^{-12}$ | - | $1.213 \times 10^{-12}$<br>$1.243 \times 10^{-12}$<br>$1.189 \times 10^{-12}$ | - | $1.129 \times 10^{0}$<br>$1.108 \times 10^{0}$<br>$1.156 \times 10^{0}$ |
| $^{123}Sn \rightarrow ^{123}Sb$ $\left[0.0, \frac{11}{2}^-\right] \rightarrow \left[1260.9, \left(\frac{9}{2}\right)^+\right]$ | $1.617 \times 10^{-13}$<br>$1.625 \times 10^{-13}$<br>$1.628 \times 10^{-13}$ | - | $7.286 \times 10^{-14}$<br>$7.241 \times 10^{-14}$<br>$7.220 \times 10^{-14}$ | - | $2.219 \times 10^{0}$<br>$2.244 \times 10^{0}$<br>$2.255 \times 10^{0}$ |

Table 2: (Cotnd.)

| Transition Details | Bound State Decay: $\lambda_B$ for R$_1$ / R$_2$ / R$_3$ in Sec$^{-1}$ | Prev. Value Takahashi | Continuum State Decay: $\lambda_C$ for R$_1$ / R$_2$ / R$_3$ in Sec$^{-1}$ | Prev. Value Takahashi | Bound to Continuum Ratio |
|---|---|---|---|---|---|
| $^{123}Sn \rightarrow ^{123}Sb$ $\left[0.0, \frac{11}{2}^-\right] \rightarrow \left[1337.4, \frac{9}{2}^+\right]$ | $3.512\times10^{-12}$<br>$3.528\times10^{-12}$<br>$3.534\times10^{-12}$ | - | $3.962\times10^{-13}$<br>$3.973\times10^{-13}$<br>$3.982\times10^{-13}$ | - | $8.864\times10^{0}$<br>$8.880\times10^{0}$<br>$8.875\times10^{0}$ |
| $^{123}Sn \rightarrow ^{123}Sb$ $\left[24.6, \frac{3}{2}^+\right] \rightarrow \left[160.3, \frac{5}{2}^+\right]$ | $1.963\times10^{-5}$<br>$1.978\times10^{-5}$<br>$1.975\times10^{-5}$ | - | $2.815\times10^{-4}$<br>$2.880\times10^{-4}$<br>$2.817\times10^{-4}$ | - | $6.973\times10^{-2}$<br>$6.868\times10^{-2}$<br>$7.011\times10^{-2}$ |
| $^{123}Sn \rightarrow ^{123}Sb$ $\left[24.6, \frac{3}{2}^+\right] \rightarrow \left[541.8, \frac{3}{2}^+\right]$ | $2.032\times10^{-8}$<br>$2.041\times10^{-8}$<br>$2.039\times10^{-8}$ | - | $1.535\times10^{-7}$<br>$1.534\times10^{-7}$<br>$1.532\times10^{-7}$ | - | $1.324\times10^{-1}$<br>$1.331\times10^{-1}$<br>$1.331\times10^{-1}$ |
| $^{123}Sn \rightarrow ^{123}Sb$ $\left[24.6, \frac{3}{2}^+\right] \rightarrow \left[712.8, \frac{1}{2}^+\right]$ | $8.932\times10^{-9}$<br>$8.980\times10^{-9}$<br>$8.990\times10^{-9}$ | - | $4.719\times10^{-8}$<br>$4.718\times10^{-8}$<br>$4.722\times10^{-8}$ | - | $1.893\times10^{-1}$<br>$1.903\times10^{-1}$<br>$1.904\times10^{-1}$ |
| $^{124}Sb \rightarrow ^{124}Te$ $[10.8627, 5^+] \rightarrow [1248.5, 4^+]$ | $1.893\times10^{-6}$<br>$1.900\times10^{-6}$<br>$1.899\times10^{-6}$ | - | $4.403\times10^{-5}$<br>$4.398\times10^{-5}$<br>$4.398\times10^{-5}$ | - | $4.299\times10^{-2}$<br>$4.320\times10^{-2}$<br>$4.318\times10^{-2}$ |
| $^{124}Sb \rightarrow ^{124}Te$ $[10.8627, 5^+] \rightarrow [1746.9, 6^+]$ | $1.542\times10^{-4}$<br>$1.551\times10^{-4}$<br>$1.551\times10^{-4}$ | - | $1.823\times10^{-3}$<br>$1.825\times10^{-3}$<br>$1.825\times10^{-3}$ | - | $8.459\times10^{-2}$<br>$8.499\times10^{-2}$<br>$8.499\times10^{-2}$ |
| $^{124}Sb \rightarrow ^{124}Te$ $[10.8627, 5^+] \rightarrow [2349.5, 6^+]$ | $1.023\times10^{-5}$<br>$1.027\times10^{-5}$<br>$1.026\times10^{-5}$ | - | $3.551\times10^{-5}$<br>$3.547\times10^{-5}$<br>$3.547\times10^{-5}$ | - | $2.881\times10^{-1}$<br>$2.895\times10^{-1}$<br>$2.893\times10^{-1}$ |
| $^{134}Cs \rightarrow ^{134}Ba$ $[0.0, 4^+] \rightarrow [1400.6, 4^+]$ | $1.921\times10^{-9}$<br>$1.944\times10^{-9}$<br>$1.915\times10^{-9}$ | - | $7.177\times10^{-9}$<br>$7.206\times10^{-9}$<br>$7.196\times10^{-9}$ | - | $2.677\times10^{-1}$<br>$2.698\times10^{-1}$<br>$2.661\times10^{-1}$ |
| $^{134}Cs \rightarrow ^{134}Ba$ $[0.0, 4^+] \rightarrow [1643.3, 3^+]$ | $1.375\times10^{-10}$<br>$1.389\times10^{-10}$<br>$1.368\times10^{-10}$ | - | $2.496\times10^{-10}$<br>$2.500\times10^{-10}$<br>$2.497\times10^{-10}$ | - | $5.509\times10^{-1}$<br>$5.556\times10^{-1}$<br>$5.479\times10^{-1}$ |
| $^{134}Cs \rightarrow ^{134}Ba$ $[0.0, 4^+] \rightarrow [1969.9, 4^+]$ | $1.469\times10^{-8}$<br>$1.480\times10^{-8}$<br>$1.461\times10^{-8}$ | - | $2.141\times10^{-9}$<br>$2.140\times10^{-9}$<br>$2.143\times10^{-9}$ | - | $6.861\times10^{0}$<br>$6.916\times10^{0}$<br>$6.818\times10^{0}$ |
| $^{136}Cs \rightarrow ^{136}Ba$ $[0.0, 5^+] \rightarrow [1866.6, 4^+]$ | $1.935\times10^{-8}$<br>$1.950\times10^{-8}$<br>$1.925\times10^{-8}$ | - | $7.654\times10^{-8}$<br>$7.650\times10^{-8}$<br>$7.656\times10^{-8}$ | - | $2.528\times10^{-1}$<br>$2.549\times10^{-1}$<br>$2.514\times10^{-1}$ |
| $^{136}Cs \rightarrow ^{136}Ba$ $[0.0, 5^+] \rightarrow [2030.5, 7^-]$ | $2.103\times10^{-10}$<br>$2.145\times10^{-10}$<br>$2.106\times10^{-10}$ | - | $5.626\times10^{-10}$<br>$5.628\times10^{-10}$<br>$5.627\times10^{-10}$ | - | $3.738\times10^{-1}$<br>$3.811\times10^{-1}$<br>$3.743\times10^{-1}$ |

Table 2: (Cotnd.)

| Transition Details | Bound State Decay: $\lambda_B$ for $R_1$ in $Sec^{-1}$ / $\lambda_B$ for $R_2$ in $Sec^{-1}$ / $\lambda_B$ for $R_3$ in $Sec^{-1}$ | Bound State Decay: Prev. Value Takahashi | Continuum State Decay: $\lambda_C$ for $R_1$ in $Sec^{-1}$ / $\lambda_C$ for $R_2$ in $Sec^{-1}$ / $\lambda_C$ for $R_3$ in $Sec^{-1}$ | Continuum State Decay: Prev. Value Takahashi | Bound to Continuum Ratio |
|---|---|---|---|---|---|
| $^{136}Cs \rightarrow ^{136}Ba$ $[0.0, 5^+] \rightarrow [2053.9, 4^+]$ | $1.148 \times 10^{-8}$ $1.157 \times 10^{-8}$ $1.140 \times 10^{-8}$ | - | $2.733 \times 10^{-8}$ $2.731 \times 10^{-8}$ $2.727 \times 10^{-8}$ | - | $4.201 \times 10^{-1}$ $4.237 \times 10^{-1}$ $4.180 \times 10^{-1}$ |
| $^{136}Cs \rightarrow ^{136}Ba$ $[0.0, 5^+] \rightarrow [2140.2, 5^-]$ | $3.400 \times 10^{-8}$ $3.426 \times 10^{-8}$ $3.383 \times 10^{-8}$ | - | $6.021 \times 10^{-8}$ $6.019 \times 10^{-8}$ $6.024 \times 10^{-8}$ | - | $5.647 \times 10^{-1}$ $5.692 \times 10^{-1}$ $5.616 \times 10^{-1}$ |
| $^{136}Cs \rightarrow ^{136}Ba$ $[0.0, 5^+] \rightarrow [2207.1, 6^+]$ | $2.939 \times 10^{-7}$ $2.963 \times 10^{-7}$ $2.926 \times 10^{-7}$ | - | $3.960 \times 10^{-7}$ $3.960 \times 10^{-7}$ $3.965 \times 10^{-7}$ | - | $7.422 \times 10^{-1}$ $7.482 \times 10^{-1}$ $7.380 \times 10^{-1}$ |
| $^{136}Cs \rightarrow ^{136}Ba$ $[0.0, 5^+] \rightarrow [2356.6, 4^+]$ | $1.995 \times 10^{-9}$ $2.010 \times 10^{-9}$ $1.985 \times 10^{-9}$ | - | $1.106 \times 10^{-9}$ $1.100 \times 10^{-9}$ $1.106 \times 10^{-9}$ | - | $1.804 \times 10^{0}$ $1.827 \times 10^{0}$ $1.795 \times 10^{0}$ |
| $^{136}Cs \rightarrow ^{136}Ba$ $[0.0, 5^+] \rightarrow [2373.7, (5)^+]$ | $2.223 \times 10^{-8}$ $2.246 \times 10^{-8}$ $2.212 \times 10^{-8}$ | - | $1.065 \times 10^{-8}$ $1.063 \times 10^{-8}$ $1.064 \times 10^{-8}$ | - | $2.087 \times 10^{0}$ $2.113 \times 10^{0}$ $2.079 \times 10^{0}$ |
| $^{148}Pm \rightarrow ^{148}Sm$ $[0.0, 1^-] \rightarrow [0.0, 0^+]$ | $2.411 \times 10^{-8}$ $2.431 \times 10^{-8}$ $2.431 \times 10^{-8}$ | - | $8.406 \times 10^{-7}$ $8.396 \times 10^{-7}$ $8.407 \times 10^{-7}$ | - | $2.868 \times 10^{-2}$ $2.895 \times 10^{-2}$ $2.892 \times 10^{-2}$ |
| $^{148}Pm \rightarrow ^{148}Sm$ $[0.0, 1^-] \rightarrow [550.3, 2^+]$ | $6.808 \times 10^{-9}$ $6.913 \times 10^{-9}$ $6.895 \times 10^{-9}$ | - | $1.410 \times 10^{-7}$ $1.418 \times 10^{-7}$ $1.416 \times 10^{-7}$ | - | $4.828 \times 10^{-2}$ $4.875 \times 10^{-2}$ $4.869 \times 10^{-2}$ |
| $^{148}Pm \rightarrow ^{148}Sm$ $[0.0, 1^-] \rightarrow [1424.5, 0^+]$ | $5.308 \times 10^{-10}$ $5.366 \times 10^{-10}$ $5.353 \times 10^{-10}$ | - | $3.499 \times 10^{-9}$ $3.503 \times 10^{-9}$ $3.499 \times 10^{-9}$ | - | $1.517 \times 10^{-1}$ $1.532 \times 10^{-1}$ $1.530 \times 10^{-1}$ |
| $^{148}Pm \rightarrow ^{148}Sm$ $[0.0, 1^-] \rightarrow [1454.2, 2^+]$ | $2.197 \times 10^{-10}$ $2.222 \times 10^{-10}$ $2.215 \times 10^{-10}$ | - | $1.376 \times 10^{-9}$ $1.378 \times 10^{-9}$ $1.377 \times 10^{-9}$ | - | $1.597 \times 10^{-1}$ $1.612 \times 10^{-1}$ $1.609 \times 10^{-1}$ |
| $^{148}Pm \rightarrow ^{148}Sm$ $[0.0, 1^-] \rightarrow [1465.1, 1^-]$ | $8.031 \times 10^{-8}$ $8.119 \times 10^{-8}$ $8.098 \times 10^{-8}$ | - | $4.942 \times 10^{-7}$ $4.948 \times 10^{-7}$ $4.943 \times 10^{-7}$ | - | $1.625 \times 10^{-1}$ $1.641 \times 10^{-1}$ $1.638 \times 10^{-1}$ |
| $^{148}Pm \rightarrow ^{148}Sm$ $[0.0, 1^-] \rightarrow [1664.2, 2^+]$ | $6.262 \times 10^{-11}$ $6.330 \times 10^{-11}$ $6.313 \times 10^{-11}$ | - | $2.639 \times 10^{-10}$ $2.642 \times 10^{-10}$ $2.640 \times 10^{-10}$ | - | $2.373 \times 10^{-1}$ $2.396 \times 10^{-1}$ $2.391 \times 10^{-1}$ |
| $^{148}Pm \rightarrow ^{148}Sm$ $[0.0, 1^-] \rightarrow [1921.6, 0^+]$ | $8.821 \times 10^{-11}$ $8.897 \times 10^{-11}$ $8.892 \times 10^{-11}$ | - | $1.986 \times 10^{-10}$ $1.984 \times 10^{-10}$ $1.986 \times 10^{-10}$ | - | $4.442 \times 10^{-1}$ $4.484 \times 10^{-1}$ $4.477 \times 10^{-1}$ |
| $^{148}Pm \rightarrow ^{148}Sm$ $[0.0, 1^-] \rightarrow [2058, 2^-]$ | $1.332 \times 10^{-8}$ $1.344 \times 10^{-8}$ $1.342 \times 10^{-8}$ | - | $1.922 \times 10^{-8}$ $1.919 \times 10^{-8}$ $1.922 \times 10^{-8}$ | - | $6.930 \times 10^{-1}$ $7.004 \times 10^{-1}$ $6.982 \times 10^{-1}$ |

Table 2: (Cotnd.)

| Transition Details | Bound State Decay: $\lambda_B$ for R$_1$ in Sec$^{-1}$ / $\lambda_B$ for R$_2$ in Sec$^{-1}$ / $\lambda_B$ for R$_3$ in Sec$^{-1}$ | Bound State Decay: Prev. Value Takahashi | Continuum State Decay: $\lambda_C$ for R$_1$ in Sec$^{-1}$ / $\lambda_C$ for R$_2$ in Sec$^{-1}$ / $\lambda_C$ for R$_3$ in Sec$^{-1}$ | Continuum State Decay: Prev. Value Takahashi | Bound to Continuum Ratio |
|---|---|---|---|---|---|
| $^{148}Pm \rightarrow ^{148}Sm$ $[0.0, 1^-] \rightarrow [2284.4, (1, 2^+)]$ | $3.268 \times 10^{-9}$ $3.303 \times 10^{-9}$ $3.294 \times 10^{-9}$ | - | $1.337 \times 10^{-9}$ $1.338 \times 10^{-9}$ $1.336 \times 10^{-9}$ | - | $2.444 \times 10^{0}$ $2.469 \times 10^{0}$ $2.466 \times 10^{0}$ |
| $^{148}Pm \rightarrow ^{148}Sm$ $[0.0, 1^-] \rightarrow [2314, 2^+]$ | $3.694 \times 10^{-10}$ $3.726 \times 10^{-10}$ $3.725 \times 10^{-10}$ | - | $1.123 \times 10^{-10}$ $1.122 \times 10^{-10}$ $1.120 \times 10^{-10}$ | - | $3.289 \times 10^{0}$ $3.321 \times 10^{0}$ $3.326 \times 10^{0}$ |
| $^{148}Pm \rightarrow ^{148}Sm$ $[137.9, 5^-, 6^-] \rightarrow [1594.3, 5^-]$ | $2.838 \times 10^{-10}$ $2.862 \times 10^{-10}$ $2.854 \times 10^{-10}$ | - | $1.773 \times 10^{-9}$ $1.771 \times 10^{-9}$ $1.769 \times 10^{-9}$ | - | $1.601 \times 10^{-1}$ $1.616 \times 10^{-1}$ $1.613 \times 10^{-1}$ |
| $^{148}Pm \rightarrow ^{148}Sm$ $[137.9, 5^-, 6^-] \rightarrow [1905.9, 6^+]$ | $1.238 \times 10^{-8}$ $1.248 \times 10^{-8}$ $1.248 \times 10^{-8}$ | - | $4.153 \times 10^{-8}$ $4.148 \times 10^{-8}$ $4.154 \times 10^{-8}$ | - | $2.981 \times 10^{-1}$ $3.009 \times 10^{-1}$ $3.001 \times 10^{-1}$ |
| $^{148}Pm \rightarrow ^{148}Sm$ $[137.9, 5^-, 6^-] \rightarrow [2095.6, 6^+]$ | $1.715 \times 10^{-8}$ $1.733 \times 10^{-8}$ $1.729 \times 10^{-8}$ | - | $3.475 \times 10^{-8}$ $3.479 \times 10^{-8}$ $3.475 \times 10^{-8}$ | - | $4.935 \times 10^{-1}$ $4.981 \times 10^{-1}$ $4.976 \times 10^{-1}$ |
| $^{148}Pm \rightarrow ^{148}Sm$ $[137.9, 5^-, 6^-] \rightarrow [2194.1, 6^+]$ | $6.822 \times 10^{-8}$ $6.881 \times 10^{-8}$ $6.877 \times 10^{-8}$ | - | $9.887 \times 10^{-8}$ $9.876 \times 10^{-8}$ $9.892 \times 10^{-8}$ | - | $6.900 \times 10^{-1}$ $6.967 \times 10^{-1}$ $6.952 \times 10^{-1}$ |
| $^{151}Sm \rightarrow ^{151}Eu$ $\left[0.0, \frac{5}{2}^-\right] \rightarrow \left[0.0, \frac{5}{2}^+\right]$ | $2.215 \times 10^{-9}$ $2.207 \times 10^{-9}$ $2.204 \times 10^{-9}$ | $2.3 \times 10^{-9}$ | $1.543 \times 10^{-10}$ $1.541 \times 10^{-10}$ $1.542 \times 10^{-10}$ | $1.5 \times 10^{-10}$ | $1.436 \times 10^{1}$ $1.432 \times 10^{1}$ $1.429 \times 10^{1}$ |
| $^{151}Sm \rightarrow ^{151}Eu$ $\left[0.0, \frac{5}{2}^-\right] \rightarrow \left[21.5, \frac{7}{2}^+\right]$ | $3.693 \times 10^{-11}$ $3.680 \times 10^{-11}$ $3.676 \times 10^{-11}$ | $3.8 \times 10^{-11}$ | $1.148 \times 10^{-12}$ $1.149 \times 10^{-12}$ $1.151 \times 10^{-12}$ | $1.1 \times 10^{-12}$ | $3.217 \times 10^{1}$ $3.203 \times 10^{1}$ $3.194 \times 10^{1}$ |
| $^{152}Eu \rightarrow ^{152}Gd$ $[0.0, 3^-] \rightarrow [344.3, 2^+]$ | $1.186 \times 10^{-11}$ $1.179 \times 10^{-11}$ $1.179 \times 10^{-11}$ | - | $1.349 \times 10^{-10}$ $1.349 \times 10^{-10}$ $1.348 \times 10^{-10}$ | - | $8.792 \times 10^{-2}$ $8.740 \times 10^{-2}$ $8.746 \times 10^{-2}$ |
| $^{152}Eu \rightarrow ^{152}Gd$ $[0.0, 3^-] \rightarrow [755.4, 4^+]$ | $2.365 \times 10^{-12}$ $2.352 \times 10^{-12}$ $2.356 \times 10^{-12}$ | - | $1.482 \times 10^{-11}$ $1.482 \times 10^{-11}$ $1.484 \times 10^{-11}$ | - | $1.596 \times 10^{-1}$ $1.587 \times 10^{-1}$ $1.588 \times 10^{-1}$ |
| $^{152}Eu \rightarrow ^{152}Gd$ $[0.0, 3^-] \rightarrow [930.5, 2^+]$ | $9.973 \times 10^{-13}$ $9.913 \times 10^{-13}$ $9.908 \times 10^{-13}$ | - | $4.568 \times 10^{-12}$ $4.568 \times 10^{-12}$ $4.564 \times 10^{-12}$ | - | $2.183 \times 10^{-1}$ $2.170 \times 10^{-1}$ $2.171 \times 10^{-1}$ |
| $^{152}Eu \rightarrow ^{152}Gd$ $[0.0, 3^-] \rightarrow [1109.2, 2^+]$ | $1.336 \times 10^{-12}$ $1.329 \times 10^{-12}$ $1.330 \times 10^{-12}$ | - | $4.201 \times 10^{-12}$ $4.200 \times 10^{-12}$ $4.206 \times 10^{-12}$ | - | $3.180 \times 10^{-1}$ $3.164 \times 10^{-1}$ $3.162 \times 10^{-1}$ |
| $^{152}Eu \rightarrow ^{152}Gd$ $[0.0, 3^-] \rightarrow [1123.2, 3^-]$ | $7.188 \times 10^{-11}$ $7.145 \times 10^{-11}$ $7.141 \times 10^{-11}$ | - | $2.189 \times 10^{-10}$ $2.188 \times 10^{-10}$ $2.186 \times 10^{-10}$ | - | $3.284 \times 10^{-1}$ $3.266 \times 10^{-1}$ $3.267 \times 10^{-1}$ |

Table 2: (Contnd.)

| Transition Details | Bound State Decay $\lambda_B$ for $R_1$ in $Sec^{-1}$ $\lambda_B$ for $R_2$ in $Sec^{-1}$ $\lambda_B$ for $R_3$ in $Sec^{-1}$ | Prev. Value Takahashi | Continuum State Decay $\lambda_C$ for $R_1$ in $Sec^{-1}$ $\lambda_C$ for $R_2$ in $Sec^{-1}$ $\lambda_C$ for $R_3$ in $Sec^{-1}$ | Prev. Value Takahashi | Bound to Continuum Ratio |
|---|---|---|---|---|---|
| $^{152}Eu \rightarrow ^{152}Gd$ $[0.0, 3^-] \rightarrow [1282.2, 4^+]$ | $1.819 \times 10^{-13}$ $1.808 \times 10^{-13}$ $1.805 \times 10^{-13}$ | - | $3.647 \times 10^{-13}$ $3.647 \times 10^{-13}$ $3.644 \times 10^{-13}$ | - | $4.988 \times 10^{-1}$ $4.957 \times 10^{-1}$ $4.953 \times 10^{-1}$ |
| $^{152}Eu \rightarrow ^{152}Gd$ $[0.0, 3^-] \rightarrow [1318.5, 2^+]$ | $1.646 \times 10^{-13}$ $1.635 \times 10^{-13}$ $1.639 \times 10^{-13}$ | - | $2.953 \times 10^{-13}$ $2.953 \times 10^{-13}$ $2.957 \times 10^{-13}$ | - | $5.574 \times 10^{-1}$ $5.537 \times 10^{-1}$ $5.543 \times 10^{-1}$ |
| $^{152}Eu \rightarrow ^{152}Gd$ $[0.0, 3^-] \rightarrow [1434, 3^+]$ | $3.129 \times 10^{-11}$ $3.111 \times 10^{-11}$ $3.116 \times 10^{-11}$ | - | $3.716 \times 10^{-11}$ $3.716 \times 10^{-11}$ $3.721 \times 10^{-11}$ | - | $8.420 \times 10^{-1}$ $8.372 \times 10^{-1}$ $8.374 \times 10^{-1}$ |
| $^{152}Eu \rightarrow ^{152}Gd$ $[0.0, 3^-] \rightarrow [1550.2, 4^+]$ | $9.928 \times 10^{-13}$ $9.868 \times 10^{-13}$ $9.863 \times 10^{-13}$ | - | $6.661 \times 10^{-13}$ $6.662 \times 10^{-13}$ $6.656 \times 10^{-13}$ | - | $1.490 \times 10^{0}$ $1.481 \times 10^{0}$ $1.482 \times 10^{0}$ |
| $^{152}Eu \rightarrow ^{152}Gd$ $[0.0, 3^-] \rightarrow [1605.6, 2^+]$ | $3.275 \times 10^{-12}$ $3.254 \times 10^{-12}$ $3.253 \times 10^{-12}$ | - | $1.514 \times 10^{-12}$ $1.514 \times 10^{-12}$ $1.512 \times 10^{-12}$ | - | $2.163 \times 10^{0}$ $2.149 \times 10^{0}$ $2.151 \times 10^{0}$ |
| $^{152}Eu \rightarrow ^{152}Gd$ $[0.0, 3^-] \rightarrow [1643.4, 2^-]$ | $7.534 \times 10^{-11}$ $7.489 \times 10^{-11}$ $7.504 \times 10^{-11}$ | - | $2.506 \times 10^{-11}$ $2.507 \times 10^{-11}$ $2.509 \times 10^{-11}$ | - | $3.006 \times 10^{0}$ $2.987 \times 10^{0}$ $2.991 \times 10^{0}$ |
| $^{152}Eu \rightarrow ^{152}Gd$ $[0.0, 3^-] \rightarrow [1692.4, 2^+, 3^+]$ | $1.346 \times 10^{-12}$ $1.338 \times 10^{-12}$ $1.341 \times 10^{-12}$ | - | $2.483 \times 10^{-13}$ $2.478 \times 10^{-13}$ $2.485 \times 10^{-13}$ | - | $5.421 \times 10^{0}$ $5.400 \times 10^{0}$ $5.396 \times 10^{0}$ |
| $^{152}Eu \rightarrow ^{152}Gd$ $[45.5998, 0^-] \rightarrow [0.0, 0^+]$ | $8.171 \times 10^{-7}$ $8.123 \times 10^{-7}$ $7.950 \times 10^{-7}$ | - | $1.466 \times 10^{-5}$ $1.466 \times 10^{-5}$ $1.434 \times 10^{-5}$ | - | $5.574 \times 10^{-2}$ $5.541 \times 10^{-2}$ $5.544 \times 10^{-2}$ |
| $^{152}Eu \rightarrow ^{152}Gd$ $[45.5998, 0^-] \rightarrow [344.3, 2^+]$ | $3.865 \times 10^{-8}$ $3.905 \times 10^{-8}$ $3.876 \times 10^{-8}$ | - | $3.433 \times 10^{-7}$ $3.441 \times 10^{-7}$ $3.439 \times 10^{-7}$ | - | $1.126 \times 10^{-1}$ $1.135 \times 10^{-1}$ $1.127 \times 10^{-1}$ |
| $^{152}Eu \rightarrow ^{152}Gd$ $[45.5998, 0^-] \rightarrow [1047.9, 0^+]$ | $4.465 \times 10^{-9}$ $4.439 \times 10^{-9}$ $4.447 \times 10^{-9}$ | - | $1.771 \times 10^{-8}$ $1.771 \times 10^{-8}$ $1.774 \times 10^{-8}$ | - | $2.521 \times 10^{-1}$ $2.506 \times 10^{-1}$ $2.507 \times 10^{-1}$ |
| $^{152}Eu \rightarrow ^{152}Gd$ $[45.5998, 0^-] \rightarrow [1314.6, 1^-]$ | $1.533 \times 10^{-7}$ $1.524 \times 10^{-7}$ $1.527 \times 10^{-7}$ | - | $3.186 \times 10^{-7}$ $3.186 \times 10^{-7}$ $3.190 \times 10^{-7}$ | - | $4.812 \times 10^{-1}$ $4.783 \times 10^{-1}$ $4.787 \times 10^{-1}$ |
| $^{152}Eu \rightarrow ^{152}Gd$ $[45.5998, 0^-] \rightarrow [1460.5, 1]$ | $1.856 \times 10^{-9}$ $1.846 \times 10^{-9}$ $1.844 \times 10^{-9}$ | - | $2.374 \times 10^{-9}$ $2.375 \times 10^{-9}$ $2.373 \times 10^{-9}$ | - | $7.818 \times 10^{-1}$ $7.773 \times 10^{-1}$ $7.771 \times 10^{-1}$ |
| $^{152}Eu \rightarrow ^{152}Gd$ $[45.5998, 0^-] \rightarrow [1756.0, 1^-]$ | $5.574 \times 10^{-8}$ $5.541 \times 10^{-8}$ $5.539 \times 10^{-8}$ | - | $7.729 \times 10^{-9}$ $7.532 \times 10^{-9}$ $7.501 \times 10^{-9}$ | - | $7.212 \times 10^{0}$ $7.357 \times 10^{0}$ $7.384 \times 10^{0}$ |

Table 2: (Contnd.)

| Transition Details | Bound State Decay: $\lambda_B$ for $R_1$ in Sec$^{-1}$ / $\lambda_B$ for $R_2$ in Sec$^{-1}$ / $\lambda_B$ for $R_3$ in Sec$^{-1}$ | Bound State Decay: Prev. Value Takahashi | Continuum State Decay: $\lambda_C$ for $R_1$ in Sec$^{-1}$ / $\lambda_C$ for $R_2$ in Sec$^{-1}$ / $\lambda_C$ for $R_3$ in Sec$^{-1}$ | Continuum State Decay: Prev. Value Takahashi | Bound to Continuum Ratio |
|---|---|---|---|---|---|
| $^{155}Eu \rightarrow ^{155}Gd$ $\left[0.0, \frac{5}{2}^+\right] \rightarrow \left[0.0, \frac{3}{2}^-\right]$ | $1.127 \times 10^{-9}$<br>$1.120 \times 10^{-9}$<br>$1.133 \times 10^{-9}$ | $9.0 \times 10^{-10}$ | $6.879 \times 10^{-10}$<br>$6.873 \times 10^{-10}$<br>$6.881 \times 10^{-10}$ | $5.8 \times 10^{-10}$ | $1.638 \times 10^{0}$<br>$1.630 \times 10^{0}$<br>$1.647 \times 10^{0}$ |
| $^{155}Eu \rightarrow ^{155}Gd$ $\left[0.0, \frac{5}{2}^+\right] \rightarrow \left[60, \frac{5}{2}^-\right]$ | $9.043 \times 10^{-10}$<br>$9.059 \times 10^{-10}$<br>$9.145 \times 10^{-10}$ | $9.2 \times 10^{-10}$ | $3.547 \times 10^{-10}$<br>$3.550 \times 10^{-10}$<br>$3.536 \times 10^{-10}$ | $3.5 \times 10^{-10}$ | $2.549 \times 10^{0}$<br>$2.552 \times 10^{0}$<br>$2.586 \times 10^{0}$ |
| $^{155}Eu \rightarrow ^{155}Gd$ $\left[0.0, \frac{5}{2}^+\right] \rightarrow \left[86.5, \frac{5}{2}^+\right]$ | $3.169 \times 10^{-9}$<br>$3.150 \times 10^{-9}$<br>$3.180 \times 10^{-9}$ | $3.3 \times 10^{-9}$ | $9.675 \times 10^{-10}$<br>$9.650 \times 10^{-10}$<br>$9.636 \times 10^{-10}$ | $9.7 \times 10^{-10}$ | $3.275 \times 10^{0}$<br>$3.264 \times 10^{0}$<br>$3.300 \times 10^{0}$ |
| $^{155}Eu \rightarrow ^{155}Gd$ $\left[0.0, \frac{5}{2}^+\right] \rightarrow \left[105.3, \frac{3}{2}^+\right]$ | $7.184 \times 10^{-9}$<br>$7.138 \times 10^{-9}$<br>$7.207 \times 10^{-9}$ | $7.6 \times 10^{-9}$ | $1.768 \times 10^{-9}$<br>$1.771 \times 10^{-9}$<br>$1.761 \times 10^{-9}$ | $1.8 \times 10^{-9}$ | $4.063 \times 10^{0}$<br>$4.030 \times 10^{0}$<br>$4.093 \times 10^{0}$ |
| $^{155}Eu \rightarrow ^{155}Gd$ $\left[0.0, \frac{5}{2}^+\right] \rightarrow \left[118, \frac{7}{2}^+\right]$ | $3.308 \times 10^{-10}$<br>$3.286 \times 10^{-10}$<br>$3.318 \times 10^{-10}$ | *$3.6 \times 10^{-9}$ | $6.901 \times 10^{-11}$<br>$6.833 \times 10^{-11}$<br>$6.817 \times 10^{-11}$ | $7.2 \times 10^{-11}$ | $4.794 \times 10^{0}$<br>$4.809 \times 10^{0}$<br>$4.867 \times 10^{0}$ |
| $^{155}Eu \rightarrow ^{155}Gd$ $\left[0.0, \frac{5}{2}^+\right] \rightarrow \left[146.1, \frac{7}{2}^-\right]$ | $1.851 \times 10^{-10}$<br>$1.839 \times 10^{-10}$<br>$1.857 \times 10^{-10}$ | $1.6 \times 10^{-10}$ | $2.442 \times 10^{-11}$<br>$2.478 \times 10^{-11}$<br>$2.464 \times 10^{-11}$ | $2.0 \times 10^{-11}$ | $7.580 \times 10^{0}$<br>$7.421 \times 10^{0}$<br>$7.537 \times 10^{0}$ |
| $^{171}Tm \rightarrow ^{171}Yb$ $\left[0.0, \frac{1}{2}^+\right] \rightarrow \left[0.0, \frac{1}{2}^-\right]$ | $9.618 \times 10^{-8}$<br>$9.766 \times 10^{-8}$<br>$9.727 \times 10^{-8}$ | $1.0 \times 10^{-7}$ | $7.404 \times 10^{-9}$<br>$7.327 \times 10^{-9}$<br>$7.286 \times 10^{-9}$ | $7.6 \times 10^{-9}$ | $1.299 \times 10^{1}$<br>$1.333 \times 10^{1}$<br>$1.335 \times 10^{1}$ |
| $^{171}Tm \rightarrow ^{171}Yb$ $\left[0.0, \frac{1}{2}^+\right] \rightarrow \left[66.7, \frac{3}{2}^-\right]$ | $2.182 \times 10^{-8}$<br>$2.211 \times 10^{-8}$<br>$2.202 \times 10^{-8}$ | $2.3 \times 10^{-8}$ | $4.076 \times 10^{-11}$<br>$4.083 \times 10^{-11}$<br>$4.001 \times 10^{-11}$ | $4.0 \times 10^{-11}$ | $5.353 \times 10^{2}$<br>$5.415 \times 10^{2}$<br>$5.503 \times 10^{2}$ |
| $^{191}Os \rightarrow ^{191}Ir$ $\left[0.0, \frac{9}{2}^-\right] \rightarrow \left[171.3, \frac{11}{2}^-\right]$ | $3.161 \times 10^{-6}$<br>$3.167 \times 10^{-6}$<br>$3.136 \times 10^{-6}$ | $3.4 \times 10^{-6}$ | $3.882 \times 10^{-7}$<br>$3.878 \times 10^{-7}$<br>$3.877 \times 10^{-7}$ | $4.0 \times 10^{-7}$ | $8.143 \times 10^{0}$<br>$8.167 \times 10^{0}$<br>$8.089 \times 10^{0}$ |

* The mismatch between $\lambda_B$ value may arise from the typographical error in the tabulation of $\lambda_B$ in Ref. Takahashi.

Table 2: (Cotnd.)

| Transition Details | Bound State Decay $\lambda_B$ for R$_1$ in Sec$^{-1}$ $\lambda_B$ for R$_2$ in Sec$^{-1}$ $\lambda_B$ for R$_3$ in Sec$^{-1}$ | Bound State Decay Prev. Value Takahashi | Continuum State Decay $\lambda_C$ for R$_1$ in Sec$^{-1}$ $\lambda_C$ for R$_2$ in Sec$^{-1}$ $\lambda_C$ for R$_3$ in Sec$^{-1}$ | Continuum State Decay Prev. Value Takahashi | Bound to Continuum Ratio |
|---|---|---|---|---|---|
| $^{207}Tl \rightarrow ^{207}Pb$ $\left[0.0, \frac{1}{2}^{+}\right] \rightarrow \left[0.0, \frac{1}{2}^{-}\right]$ | $4.098\times10^{-4}$ $4.122\times10^{-4}$ $4.159\times10^{-4}$ | * | $2.530\times10^{-3}$ $2.526\times10^{-3}$ $2.529\times10^{-3}$ | * | $1.620\times10^{-1}$ $1.632\times10^{-1}$ $1.645\times10^{-1}$ |
| $^{207}Tl \rightarrow ^{207}Pb$ $\left[0.0, \frac{1}{2}^{+}\right] \rightarrow \left[569.6, \frac{5}{2}^{-}\right]$ | $5.078\times10^{-10}$ $5.238\times10^{-10}$ $5.179\times10^{-10}$ | - | $9.159\times10^{-10}$ $9.174\times10^{-10}$ $9.152\times10^{-10}$ | - | $5.544\times10^{-1}$ $5.710\times10^{-1}$ $5.659\times10^{-1}$ |
| $^{207}Tl \rightarrow ^{207}Pb$ $\left[0.0, \frac{1}{2}^{+}\right] \rightarrow \left[897.8, \frac{3}{2}^{-}\right]$ | $5.828\times10^{-6}$ $5.876\times10^{-6}$ $5.917\times10^{-6}$ | - | $6.403\times10^{-6}$ $6.409\times10^{-6}$ $6.401\times10^{-6}$ | - | $9.102\times10^{-1}$ $9.168\times10^{-1}$ $9.244\times10^{-1}$ |
| $^{210}Pb \rightarrow ^{210}Bi$ $\left[0.0, 0^{+}\right] \rightarrow \left[0.0, 1^{-}\right]$ | $5.886\times10^{-9}$ $5.917\times10^{-9}$ $5.979\times10^{-9}$ | $7.5\times10^{-9}$ | $1.739\times10^{-10}$ $1.734\times10^{-10}$ $1.738\times10^{-10}$ | $7.7\times10^{-11}$ | $3.385\times10^{1}$ $3.412\times10^{1}$ $3.440\times10^{1}$ |
| $^{210}Pb \rightarrow ^{210}Bi$ $\left[0.0, 0^{+}\right] \rightarrow \left[46.5, 0^{-}\right]$ | $7.768\times10^{-7}$ $7.826\times10^{-7}$ $7.888\times10^{-7}$ | $8.3\times10^{-7}$ | 0 | 0 | $\infty$ |
| $^{228}Ra \rightarrow ^{228}Ac$ $\left[0.0, 0^{+}\right] \rightarrow \left[6.3, 1^{-}\right]$ | $5.899\times10^{-8}$ - $5.848\times10^{-8}$ | - | $5.026\times10^{-11}$ - $5.044\times10^{-11}$ | - | $1.174\times10^{3}$ - $1.159\times10^{3}$ |
| $^{228}Ra \rightarrow ^{228}Ac$ $\left[0.0, 0^{+}\right] \rightarrow \left[6.7, 1^{+}\right]$ | $2.346\times10^{-7}$ - $2.325\times10^{-7}$ | $2.3\times10^{-7}$ | $1.870\times10^{-10}$ - $1.862\times10^{-10}$ | $1.8\times10^{-10}$ | $1.255\times10^{3}$ - $1.249\times10^{3}$ |
| $^{228}Ra \rightarrow ^{228}Ac$ $\left[0.0, 0^{+}\right] \rightarrow \left[20.2, 1^{-}\right]$ | $3.503\times10^{-7}$ - $3.474\times10^{-7}$ | - | $8.970\times10^{-12}$ - $8.957\times10^{-12}$ | - | $3.936\times10^{4}$ - $3.879\times10^{4}$ |
| $^{228}Ra \rightarrow ^{228}Ac$ $\left[0.0, 0^{+}\right] \rightarrow \left[33.1, 1^{+}\right]$ | $3.400\times10^{-6}$ - $3.370\times10^{-6}$ | $4.9\times10^{-6}$ | 0 | 0 | $\infty$ |

* Experimentally available values are given in IIIB of the main manuscript.

Table 2: (Cotnd.)

| Transition Details | Bound State Decay | | Continuum State Decay | | Bound to Continuum Ratio |
|---|---|---|---|---|---|
| | $\lambda_B$ for R$_1$ in Sec$^{-1}$<br>$\lambda_B$ for R$_2$ in Sec$^{-1}$<br>$\lambda_B$ for R$_3$ in Sec$^{-1}$ | Prev. Value<br>Takahashi | $\lambda_C$ for R$_1$ in Sec$^{-1}$<br>$\lambda_C$ for R$_2$ in Sec$^{-1}$<br>$\lambda_C$ for R$_3$ in Sec$^{-1}$ | Prev. Value<br>Takahashi | |
| $^{227}Ac \rightarrow ^{227}Th$<br>$\left[0.0, \frac{3}{2}^{-}\right] \rightarrow \left[0.0, \left(\frac{1}{2}^{+}\right)\right]$ | 6.439 $\times 10^{-8}$<br>6.504 $\times 10^{-8}$<br>6.393 $\times 10^{-8}$ | 7.2 $\times 10^{-8}$ | 1.039 $\times 10^{-10}$<br>1.038 $\times 10^{-10}$<br>1.040 $\times 10^{-10}$ | 9.8 $\times 10^{-11}$ | 6.197 $\times 10^{2}$<br>6.266 $\times 10^{2}$<br>6.147 $\times 10^{2}$ |
| $^{227}Ac \rightarrow ^{227}Th$<br>$\left[0.0, \frac{3}{2}^{-}\right] \rightarrow \left[9.3, \left(\frac{5}{2}^{+}\right)\right]$ | 7.626 $\times 10^{-8}$<br>7.686 $\times 10^{-8}$<br>7.555 $\times 10^{-8}$ | 8.3 $\times 10^{-8}$ | 3.184 $\times 10^{-11}$<br>3.209 $\times 10^{-11}$<br>3.213 $\times 10^{-11}$ | 2.9 $\times 10^{-11}$ | 2.395 $\times 10^{3}$<br>2.395 $\times 10^{3}$<br>2.419 $\times 10^{3}$ |
| $^{227}Ac \rightarrow ^{227}Th$<br>$\left[0.0, \frac{3}{2}^{-}\right] \rightarrow \left[24.5, \left(\frac{3}{2}^{+}\right)\right]$ | 8.899 $\times 10^{-8}$<br>8.968 $\times 10^{-8}$<br>8.815 $\times 10^{-8}$ | 1.1 $\times 10^{-7}$ | 1.742 $\times 10^{-15}$<br>1.740 $\times 10^{-15}$<br>1.741$\times 10^{-15}$ | 0 | 5.108 $\times 10^{7}$<br>5.154 $\times 10^{7}$<br>5.063 $\times 10^{7}$ |
| $^{227}Ac \rightarrow ^{227}Th$<br>$\left[0.0, \frac{3}{2}^{-}\right] \rightarrow \left[37.9, \left(\frac{3}{2}^{-}\right)\right]$ | 4.968 $\times 10^{-8}$<br>5.018 $\times 10^{-8}$<br>4.933 $\times 10^{-8}$ | - | 0 | - | $\infty$ |
| $^{241}Pu \rightarrow ^{241}Am$<br>$\left[0.0, \frac{5}{2}^{+}\right] \rightarrow \left[0.0, \frac{5}{2}^{-}\right]$ | 1.687 $\times 10^{-6}$<br>1.699 $\times 10^{-6}$<br>1.724 $\times 10^{-6}$ | 1.9 $\times 10^{-6}$ | 0 | 0 | $\infty$ |

Table 3: Comparison of Neutral Atom and Bare Atom $\beta^-$ Decay Rate for Radius $R_1$.

| Transition Details | | $\beta^-$ Decay half-life | | $\frac{\lambda_{Bare}(=\lambda_B+\lambda_C)}{\lambda_{Neutral}}$ |
|---|---|---|---|---|
| Parent | Daughter Levels | Neutral Atom (NNDC) | Bare Atom (Present Calculation) | |
| $^{63}Ni\left[0.0, \frac{1}{2}^-\right]$ | $^{63}Cu\left[0.0, \frac{3}{2}^-\right]$ | 101.2 years | 47.177 years | $2.15 \times 10^0$ |
| $^{66}Ni\ [0.0, 0^+]$ | $^{66}Cu[0.0, 1^+]$ | 54.6 hours | 45.729 hours | $1.19 \times 10^0$ |
| $^{85}Kr\left[0.0, \frac{9}{2}^+\right]$ | $^{85}Rb\left[0.0, \frac{5}{2}^-\right]$ | 10.739 years | 5.488 years | $1.05 \times 10^0$ |
| | $^{85}Rb\left[514.0, \frac{9}{2}^+\right]$ | | | $1.58 \times 10^0$ |
| $^{85}Kr\left[304.86, \frac{1}{2}^-\right]$ | $^{85}Rb\left[151.2, \frac{3}{2}^-\right]$ | 5.683 hours | 5.426 hours | $1.05 \times 10^0$ |
| | $^{85}Rb\left[281.0, \frac{1}{2}^-\right]$ | | | $1.07 \times 10^0$ |
| | $^{85}Rb\left[731.9, \frac{3}{2}^-\right]$ | | | $1.34 \times 10^0$ |
| $^{93}Zr\left[0.0, \frac{5}{2}^+\right]$ | $^{93}Nb\left[30.8, \frac{1}{2}^-\right]$ | $2.205\times10^6$ years | $1.690 \times 10^6$ years | $1.31 \times 10^0$ |

Table 3: (Cotnd.)

| Transition Details | | $\beta^-$ Decay half-life | | $\frac{\lambda_{Bare}(=\lambda_B+\lambda_C)}{\lambda_{Neutral}}$ |
|---|---|---|---|---|
| Parent | Daughter Levels | Neutral Atom (NNDC) | Bare Atom (Present Calculation) | |
| $^{95}Nb\left[0.0, \frac{9}{2}^+\right]$ | $^{95}Mo\left[765.8, \frac{7}{2}^+\right]$ | 35.002 days | 18.532 days | $1.89\times10^0$ |
| $^{95}Nb\left[234.7, \frac{1}{2}^-\right]$ | $^{95}Mo\left[0.0, \frac{5}{2}^+\right]$ | 63.653 days | 61.163 days | $1.03\times10^0$ |
| | $^{95}Mo\left[204.1, \frac{5}{2}^+\right]$ | | | $1.05\times10^0$ |
| | $^{95}Mo\left[786.2, \frac{5}{2}^+\right]$ | | | $1.27\times10^0$ |
| | $^{95}Mo\left[820.6, \frac{3}{2}^+\right]$ | | | $1.31\times10^0$ |
| | $^{95}Mo\left[1039.3, \frac{1}{2}^+\right]$ | | | $2.31\times10^0$ |
| $^{99}Tc\left[142.7, \frac{1}{2}^-\right]$ | $^{99}Ru\left[0.0, \frac{5}{2}^+\right]$ | 18.532 years | 14.077 years | $1.15\times10^0$ |
| | $^{99}Ru\left[89.6, \frac{3}{2}^+\right]$ | | | $1.32\times10^0$ |
| | $^{99}Ru\left[322.4, \frac{3}{2}^+\right]$ | | | $2.54\times10^0$ |

Table 3: (Cotnd.)

| Transition Details | | $\beta^-$ Decay half-life | | $\frac{\lambda_{Bare}(=\lambda_B+\lambda_C)}{\lambda_{Neutral}}$ |
|---|---|---|---|---|
| Parent | Daughter Levels | Neutral Atom (NNDC) | Bare Atom (Present Calculation) | |
| $^{106}Ru\ [0.0, 0^+]$ | $^{106}Rh\ [0.0, 1^+]$ | 371.8 days | 37.745 days | 9.85 $\times 10^0$ |
| $^{107}Pd\left[0.0, \frac{5}{2}^+\right]$ | $^{107}Ag\left[0.0, \frac{1}{2}^-\right]$ | 6.5$\times 10^6$ years | 3.628 $\times 10^6$ years | 1.79 $\times 10^0$ |
| $^{110}Ag\ [117.59, 6^+]$ | $^{110}Cd\ [2479.9, 6^+]$ | 0.694 years | 76.902 days | 1.21 $\times 10^0$ |
| | $^{110}Cd\ [2539.7, 5^-]$ | | | 1.26 $\times 10^0$ |
| | $^{110}Cd\ [2659.9, 5^-]$ | | | 1.40 $\times 10^0$ |
| | $^{110}Cd\ [2842.6, (5)^-]$ | | | 2.13 $\times 10^0$ |
| | $^{110}Cd\ [2876.8, 6^+]$ | | | 2.59 $\times 10^0$ |
| | $^{110}Cd\ [2926.7, 5^+]$ | | | 4.17 $\times 10^0$ |
| $^{113}Cd\left[263.7, \frac{11}{2}^-\right]$ | $^{113}In\left[0.0, \frac{9}{2}^+\right]$ | 14.103 years | 11.898 years | 1.19 $\times 10^0$ |

Table 3: (Cotnd.)

| Transition Details | | $\beta^-$ Decay half-life | | $\frac{\lambda_{Bare}(=\lambda_B+\lambda_C)}{\lambda_{Neutral}}$ |
|---|---|---|---|---|
| Parent | Daughter Levels | Neutral Atom (NNDC) | Bare Atom (Present Calculation) | |
| $^{115}Cd\left[181.0, \frac{11}{2}^-\right]$ | $^{115}In\left[0.0, \frac{9}{2}^+\right]$ | 44.56 days | 43.379 days | $1.02\times10^0$ |
| | $^{115}In\left[933.8, \frac{7}{2}^+\right]$ | | | $1.12\times10^0$ |
| | $^{115}In\left[1132.6, \frac{11}{2}^+\right]$ | | | $1.24\times10^0$ |
| | $^{115}In\left[1290.6, \frac{13}{2}^+\right]$ | | | $1.43\times10^0$ |
| | $^{115}In\left[1418.3, \left(\frac{9}{2}\right)^+\right]$ | | | $1.86\times10^0$ |
| | $^{115}In\left[1448.8, \frac{9}{2}^+\right]$ | | | $2.09\times10^0$ |
| | $^{115}In\left[1486.1, \frac{9}{2}^+\right]$ | | | $2.50\times10^0$ |
| $^{121}Sn\left[0.0, \frac{3}{2}^+\right]$ | $^{121}Sb\left[0.0, \frac{5}{2}^+\right]$ | 27.03 hours | 19.437 hours | $1.39\times10^0$ |
| $^{121}Sn\left[6.3, \frac{11}{2}^-\right]$ | $^{121}Sb\left[37.2, \frac{7}{2}^+\right]$ | 195.982 years | 100.969 years | $1.94\times10^0$ |

Table 3: (Cotnd.)

| Transition Details | | $\beta^-$ Decay half-life | | $\frac{\lambda_{Bare}(=\lambda_B+\lambda_C)}{\lambda_{Neutral}}$ |
|---|---|---|---|---|
| Parent | Daughter Levels | Neutral Atom (NNDC) | Bare Atom (Present Calculation) | |
| $^{123}Sn\left[0.0, \frac{11}{2}^-\right]$ | $^{123}Sb\left[0.0, \frac{7}{2}^+\right]$ | 129.2 days | 124.027 days | 1.04 $\times 10^0$ |
| | $^{123}Sb\left[1030.2, \frac{9}{2}^+\right]$ | | | 1.42 $\times 10^0$ |
| | $^{123}Sb\left[1088.7, \left(\frac{9}{2}\right)^+\right]$ | | | 1.54 $\times 10^0$ |
| | $^{123}Sb\left[1181.3, \left(\frac{9}{2}\right)^+\right]$ | | | 1.89 $\times 10^0$ |
| | $^{123}Sb\left[1260.9, \left(\frac{9}{2}\right)^+\right]$ | | | 2.70 $\times 10^0$ |
| | $^{123}Sb\left[1337.4, \frac{9}{2}^+\right]$ | | | 6.42 $\times 10^0$ |
| $^{123}Sn\left[24.6, \frac{3}{2}^+\right]$ | $^{123}Sb\left[160.3, \frac{5}{2}^+\right]$ | 40.06 minutes | 38.334 minutes | 1.05 $\times 10^0$ |
| | $^{123}Sb\left[541.8, \frac{3}{2}^+\right]$ | | | 1.10 $\times 10^0$ |
| | $^{123}Sb\left[712.8, \frac{1}{2}^+\right]$ | | | 1.15 $\times 10^0$ |

Table 3: (Cotnd.)

| Transition Details | | $\beta^-$ Decay half-life | | $\frac{\lambda_{Bare}(=\lambda_B+\lambda_C)}{\lambda_{Neutral}}$ |
|---|---|---|---|---|
| Parent | Daughter Levels | Neutral Atom (NNDC) | Bare Atom (Present Calculation) | |
| $^{124}Sb$ $[10.8627, 5^+]$ | $^{124}Te$ $[1248.5, 4^+]$ | 356.322 seconds | 334.999 seconds | $1.03\ \times10^0$ |
| | $^{124}Te$ $[1746.9, 6^+]$ | | | $1.06\ \times10^0$ |
| | $^{124}Te$ $[2349.5, 6^+]$ | | | $1.23\ \times10^0$ |
| $^{134}Cs$ $[0.0, 4^+]$ | $^{134}Ba[1400.6, 4^+]$ | 2.066 years | 304.800 days | $1.22\ \times10^0$ |
| | $^{134}Ba[1643.3, 3^+]$ | | | $1.46\ \times10^0$ |
| | $^{134}Ba[1969.9, 4^+]$ | | | $5.80\ \times10^0$ |

Table 3: (Cotnd.)

| Transition Details | | $\beta^-$ Decay half-life | | $\frac{\lambda_{Bare}(=\lambda_B+\lambda_C)}{\lambda_{Neutral}}$ |
|---|---|---|---|---|
| Parent | Daughter Levels | Neutral Atom (NNDC) | Bare Atom (Present Calculation) | |
| $^{136}Cs$ $[0.0, 5^+]$ | $^{136}Ba[1866.6, 4^+]$ | 13.16 days | 8.375 days | 1.21 $\times 10^0$ |
| | $^{136}Ba[2030.5, 7^-]$ | | | 1.27 $\times 10^0$ |
| | $^{136}Ba[2053.9, 4^+]$ | | | 1.36 $\times 10^0$ |
| | $^{136}Ba[2140.2, 5^-]$ | | | 1.47 $\times 10^0$ |
| | $^{136}Ba[2207.1, 6^+]$ | | | 1.61 $\times 10^0$ |
| | $^{136}Ba[2356.6, 4^+]$ | | | 2.42 $\times 10^0$ |
| | $^{136}Ba[2373.7, 5^+]$ | | | 2.65 $\times 10^0$ |

Table 3: (Cotnd.)

| Transition Details | | $\beta^-$ Decay half-life | | $\frac{\lambda_{Bare}(=\lambda_B+\lambda_C)}{\lambda_{Neutral}}$ |
|---|---|---|---|---|
| Parent | Daughter Levels | Neutral Atom (NNDC) | Bare Atom (Present Calculation) | |
| $^{148}Pm\ [0.0, 1^-]$ | $^{148}Sm\ [0.0, 0^+]$ | 5.368 days | 4.918 days | $1.04\ \times 10^0$ |
| | $^{148}Sm\ [550.3, 2^+]$ | | | $1.05\ \times 10^0$ |
| | $^{148}Sm\ [1424.5, 0^+]$ | | | $1.14\ \times 10^0$ |
| | $^{148}Sm\ [1454.2, 2^+]$ | | | $1.15\ \times 10^0$ |
| | $^{148}Sm\ [1465.1, 1^-]$ | | | $1.15\ \times 10^0$ |
| | $^{148}Sm\ [1664.2, 2^+]$ | | | $1.21\ \times 10^0$ |
| | $^{148}Sm\ [1921.6, 0^+]$ | | | $1.39\ \times 10^0$ |
| | $^{148}Sm\ [2058, 2^-]$ | | | $1.60\ \times 10^0$ |
| | $^{148}Sm\ [2284.4, (1, 2^+)]$ | | | $3.21\ \times 10^0$ |
| | $^{148}Sm\ [2314, 2^+]$ | | | $3.54\ \times 10^0$ |

Table 3: (Cotnd.)

| Transition Details | | $\beta^-$ Decay half-life | | $\frac{\lambda_{Bare}(=\lambda_B+\lambda_C)}{\lambda_{Neutral}}$ |
|---|---|---|---|---|
| Parent | Daughter Levels | Neutral Atom (NNDC) | Bare Atom (Present Calculation) | |
| $^{148}Pm$ $[137.9, 5^-, 6^-]$ | $^{148}Sm$ $[1594.3, 5^-]$ | 43.227 days | 29.167 days | 1.15 $\times 10^0$ |
| | $^{148}Sm$ $[1905.9, 6^+]$ | | | 1.27 $\times 10^0$ |
| | $^{148}Sm$ $[2095.6, 6^+]$ | | | 1.43 $\times 10^0$ |
| | $^{148}Sm$ $[2194.1, 6^+]$ | | | 1.59 $\times 10^0$ |
| $^{151}Sm$ $\left[0.0, \frac{5}{2}^-\right]$ | $^{151}Eu\left[0.0, \frac{5}{2}^+\right]$ | 90 years | 9.130 years | 9.79 $\times 10^0$ |
| | $^{151}Eu\left[21.5, \frac{7}{2}^+\right]$ | | | 1.71 $\times 10^1$ |

Table 3: (Cotnd.)

| Transition Details | | $\beta^-$ Decay half-life | | $\frac{\lambda_{Bare}(=\lambda_B+\lambda_C)}{\lambda_{Neutral}}$ |
|---|---|---|---|---|
| Parent | Daughter Levels | Neutral Atom (NNDC) | Bare Atom (Present Calculation) | |
| $^{152}Eu$ $[0.0, 3^-]$ | $^{152}Gd$ $[344.3, 2^+]$ | 48.437 years | 34.137 years | 1.10 $\times 10^0$ |
| | $^{152}Gd$ $[755.4, 4^+]$ | | | 1.16 $\times 10^0$ |
| | $^{152}Gd$ $[930.5, 2^+]$ | | | 1.21 $\times 10^0$ |
| | $^{152}Gd$ $[1109.2, 2^+]$ | | | 1.29 $\times 10^0$ |
| | $^{152}Gd$ $[1123.2, 3^-]$ | | | 1.30 $\times 10^0$ |
| | $^{152}Gd$ $[1282.2, 4^+]$ | | | 1.45 $\times 10^0$ |
| | $^{152}Gd$ $[1318.5, 2^+]$ | | | 1.50 $\times 10^0$ |
| | $^{152}Gd$ $[1434, 3^+]$ | | | 1.73 $\times 10^0$ |
| | $^{152}Gd$ $[1550.2, 4^+]$ | | | 2.24 $\times 10^0$ |
| | $^{152}Gd$ $[1605.6, 2^+]$ | | | 2.76 $\times 10^0$ |
| | $^{152}Gd$ $[1643.4, 2^-]$ | | | 3.37 $\times 10^0$ |
| | $^{152}Gd$ $[1692.4, 2^+3^+]$ | | | 4.94 $\times 10^0$ |

Table 3: (Cotnd.)

| Transition Details | | $\beta^-$ Decay half-life | | $\frac{\lambda_{Bare}(=\lambda_B+\lambda_C)}{\lambda_{Neutral}}$ |
|---|---|---|---|---|
| Parent | Daughter Levels | Neutral Atom (NNDC) | Bare Atom (Present Calculation) | |
| $^{152}Eu\ [45.5998, 0^-]$ | $^{152}Gd\ [0.0, 0^+]$ | 12.678 hours | 11.724 hours | 1.07 $\times 10^0$ |
| | $^{152}Gd\ [344.3, 2^+]$ | | | 1.09 $\times 10^0$ |
| | $^{152}Gd\ [1047.9, 0^+]$ | | | 1.23 $\times 10^0$ |
| | $^{152}Gd\ [1314.6, 1^-]$ | | | 1.43 $\times 10^0$ |
| | $^{152}Gd\ [1460.5, 1, 2^+]$ | | | 1.68 $\times 10^0$ |
| | $^{152}Gd\ [1756.0, 1^-]$ | | | 6.14 $\times 10^0$ |
| $^{155}Eu\ \left[0.0, \frac{5}{2}^+\right]$ | $^{155}Gd\left[0.0, \frac{3}{2}^-\right]$ | 4.753 years | 1.310 years | 2.35 $\times 10^0$ |
| | $^{155}Gd\left[60.0, \frac{5}{2}^-\right]$ | | | 3.03 $\times 10^0$ |
| | $^{155}Gd\left[86.5, \frac{5}{2}^+\right]$ | | | 3.58 $\times 10^0$ |
| | $^{155}Gd\left[105.3, \frac{3}{2}^+\right]$ | | | 4.12 $\times 10^0$ |
| | $^{155}Gd\left[118.0, \frac{7}{2}^+\right]$ | | | 4.55 $\times 10^0$ |
| | $^{155}Gd\left[146.1, \frac{7}{2}^-\right]$ | | | 6.21 $\times 10^0$ |

Table 3: (Cotnd.)

| Transition Details | | $\beta^-$ Decay half-life | | $\frac{\lambda_{Bare}(=\lambda_B+\lambda_C)}{\lambda_{Neutral}}$ |
|---|---|---|---|---|
| Parent | Daughter Levels | Neutral Atom (NNDC) | Bare Atom (Present Calculation) | |
| $^{171}Tm\left[0.0,\frac{1}{2}^+\right]$ | $^{171}Yb\left[0.0,\frac{1}{2}^-\right]$ | 1.92 years | 63.931 days | 9.23 $\times 10^0$ |
| | $^{171}Yb\left[66.7,\frac{3}{2}^-\right]$ | | | 9.55 $\times 10^1$ |
| $^{191}Os\left[0.0,\frac{9}{2}^-\right]$ | $^{191}Ir\left[171.3,\frac{11}{2}^-\right]$ | 15.4 days | 2.260 days | 6.82 $\times 10^0$ |
| $^{207}Tl\left[0.0,\frac{1}{2}^+\right]$ | $^{207}Pb\left[0.0,\frac{1}{2}^-\right]$ | 4.77 minutes | 3.912 minutes | 1.22 $\times 10^0$ |
| | $^{207}Pb\left[569.6,\frac{5}{2}^-\right]$ | | | 1.47 $\times 10^0$ |
| | $^{207}Pb\left[897.8,\frac{3}{2}^-\right]$ | | | 1.86 $\times 10^0$ |
| $^{210}Pb\left[0.0,0^+\right]$ | $^{210}Bi\left[0.0,1^-\right]$ | 22.20 years | 10.245 days | 3.83 $\times 10^1$ |
| | $^{210}Bi\left[46.5,0^-\right]$ | | | 1.69 $\times 10^3$ |

Table 3: (Cotnd.)

| Transition Details | | β⁻ Decay half-life | | $\frac{\lambda_{Bare}(=\lambda_B+\lambda_C)}{\lambda_{Neutral}}$ |
|---|---|---|---|---|
| Parent | Daughter Levels | Neutral Atom (NNDC) | Bare Atom (Present Calculation) | |
| $^{228}Ra\ [0.0, 0^+]$ | $^{228}Ac\ [6.3, 1^-]$ | 5.75 years | 1.983 days | $1.55\ \times 10^2$ |
| | $^{228}Ac\ [6.7, 1^+]$ | | | $1.54\ \times 10^2$ |
| | $^{228}Ac\ [20.2, 1^-]$ | | | $4.58\ \times 10^2$ |
| | $^{228}Ac\ [33.1, 1^+]$ | | | $2.96\ \times 10^3$ |
| $^{227}Ac\ \left[0.0, \frac{3}{2}^-\right]$ | $^{227}Th\ \left[0.0, \left(\frac{1}{2}^+\right)\right]$ | 21.926 years | 28.701 days | $1.18\ \times 10^2$ |
| | $^{227}Th\ \left[9.3, \left(\frac{5}{2}^+\right)\right]$ | | | $2.16\ \times 10^2$ |
| | $^{227}Th\ \left[24.5, \left(\frac{3}{2}^+\right)\right]$ | | | $8.82\ \times 10^2$ |
| | $^{227}Th\ \left[37.9, \left(\frac{3}{2}^-\right)\right]$ | | | $1.65\ \times 10^4$ |
| $^{241}Pu\ \left[0.0, \frac{5}{2}^+\right]$ | $^{241}Am\left[0.0, \frac{5}{2}^-\right]$ | 14.329 years | 4.755 days | $1.10\ \times 10^0$ |
